# Supplementary material for: Local Number Fluctuations in Hyperuniform and Nonhyperuniform Systems: Higher-Order Moments and Distribution Functions
Source: arXiv:2012.02358 ancillary file (2020-12-07)
Supplement: Supplementary file 1 [file SM.pdf]

# Supplementary Material — Local Number Fluctuations in Hyperuniform and Nonhyperuniform Systems: Higher-Order Moments and Distribution Functions

Salvatore Torquato\*

*Department of Physics, Princeton University, Princeton, NJ 08544, USA and  
Department of Chemistry, Princeton Institute for the Science and Technology of Materials,  
and Program in Applied and Computational Mathematics,  
Princeton University, Princeton, New Jersey 08544, USA*

Jaeuk Kim<sup>†</sup> and Michael A. Klatt<sup>‡</sup>

*Department of Physics, Princeton University, Princeton, NJ 08544, USA*

(Dated: December 3, 2020)

## I. GENERAL LOCAL MOMENT FORMULAS AND PROBABILITY DISTRIBUTION FOR HOMOGENEOUS POINT PROCESSES

Here, we present the theoretical predictions that we discussed in Sec. III in the main article.

### A. Moments

Here, we demonstrate that the bounds on the third and fourth cumulants described in Sec. IIIA can be relatively sharp for sufficiently small values of  $R$ . Figure S1 compares the simulation results of the skewness  $\gamma_1(R)$  and its lower bound [Eq. (29) in the main article] for all models considered in this work. Figure S2 compares our simulation estimates of the excess kurtosis  $\gamma_2(R)$  to corresponding lower bounds [Eqs. (30) and (33) in the main article] for all models considered in this work. To evaluate the bounds, we use our numerical estimates of the first four moments (or cumulants) with the only exception of the simple cubic lattice in 3D for  $R < 0.5$ . In that case, the moments are numerically difficult to evaluate. Therefore, we present formulas from Sec. IIIC for  $R < 0.5$ .

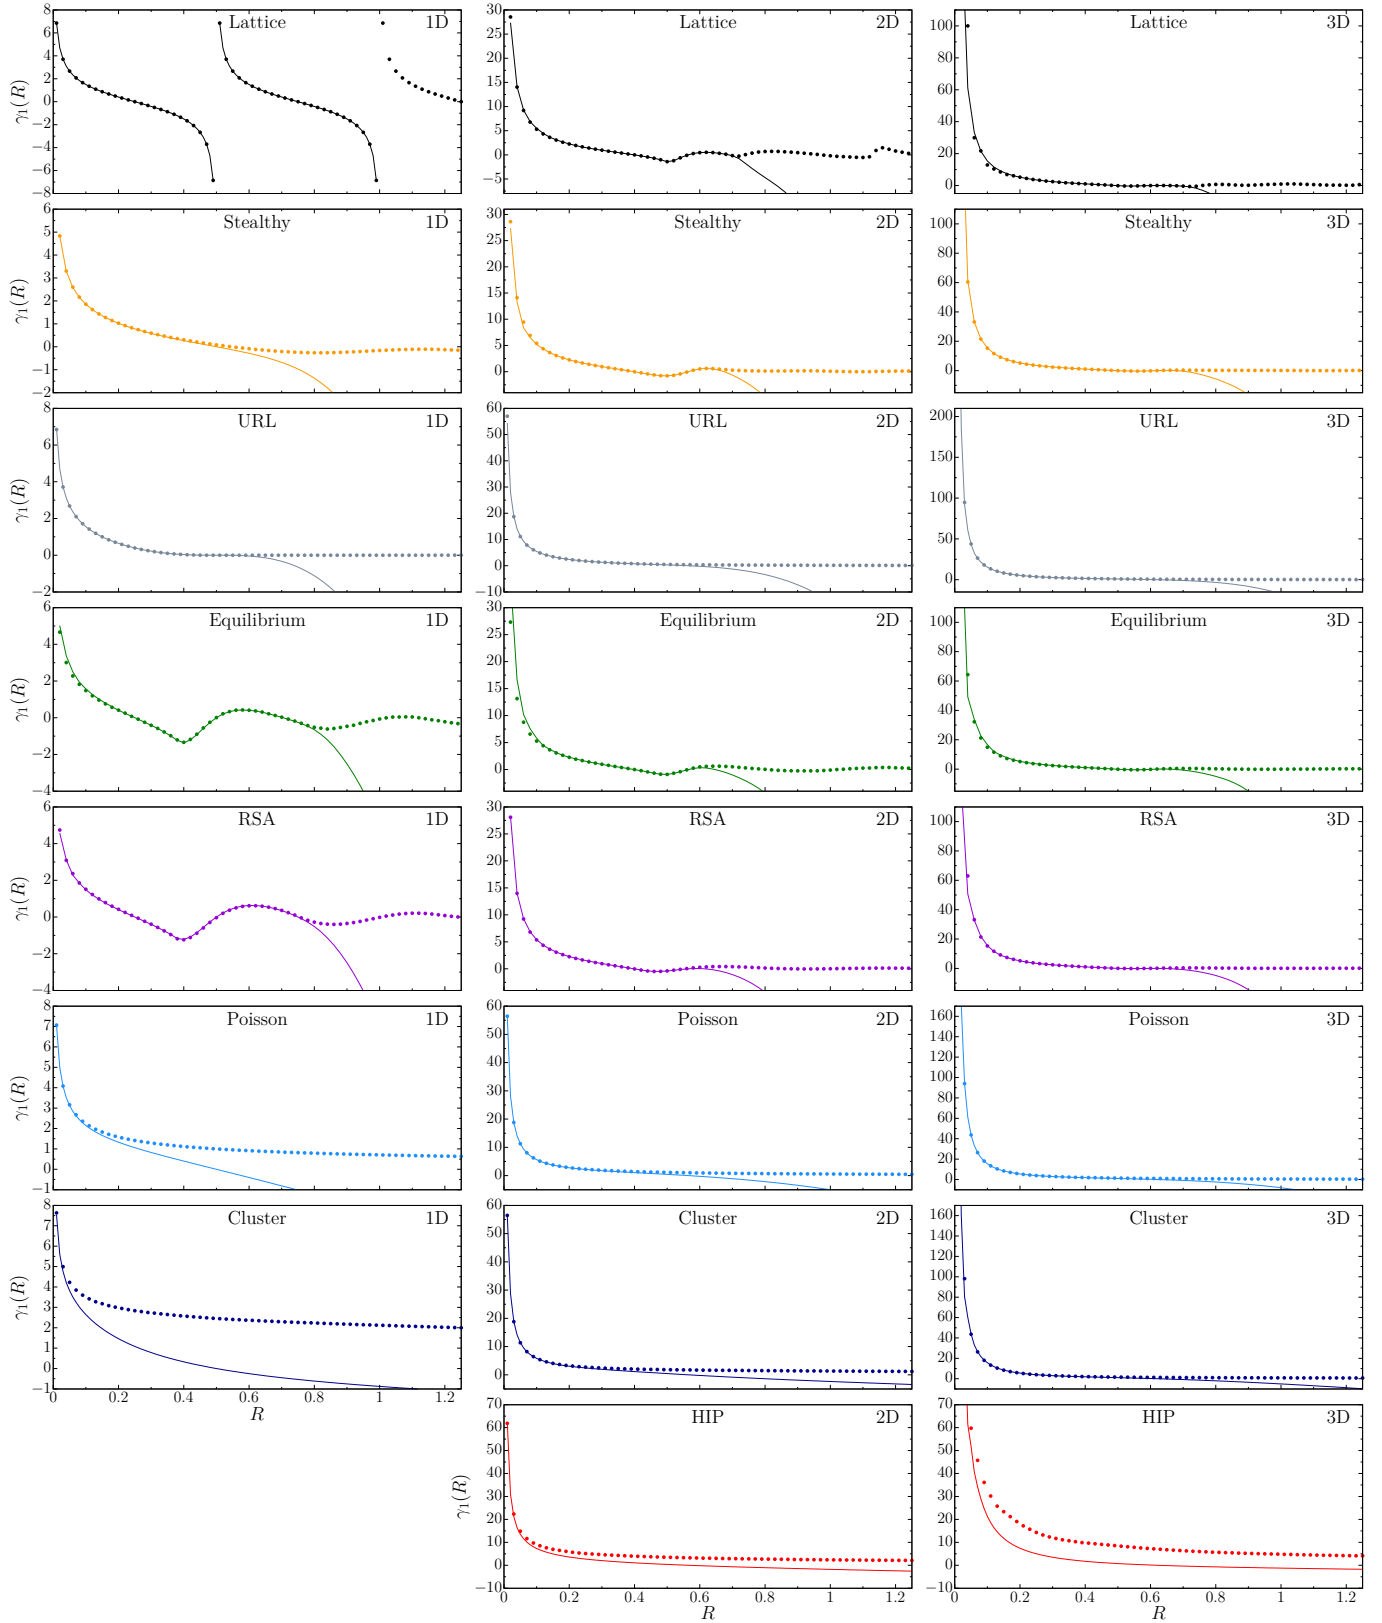

FIG. S1. Simulation results of the skewness  $\gamma_1(R)$  and their lower bounds, given in Eq. (29) in the main article, for all models considered in this paper. The dotted lines represent the simulation results, and the solid lines stand for their lower bounds. To evaluate the lower bounds, we employ the simulation results of the number variance  $\sigma^2(R)$ . The bounds are very sharp for small values of  $R$ .

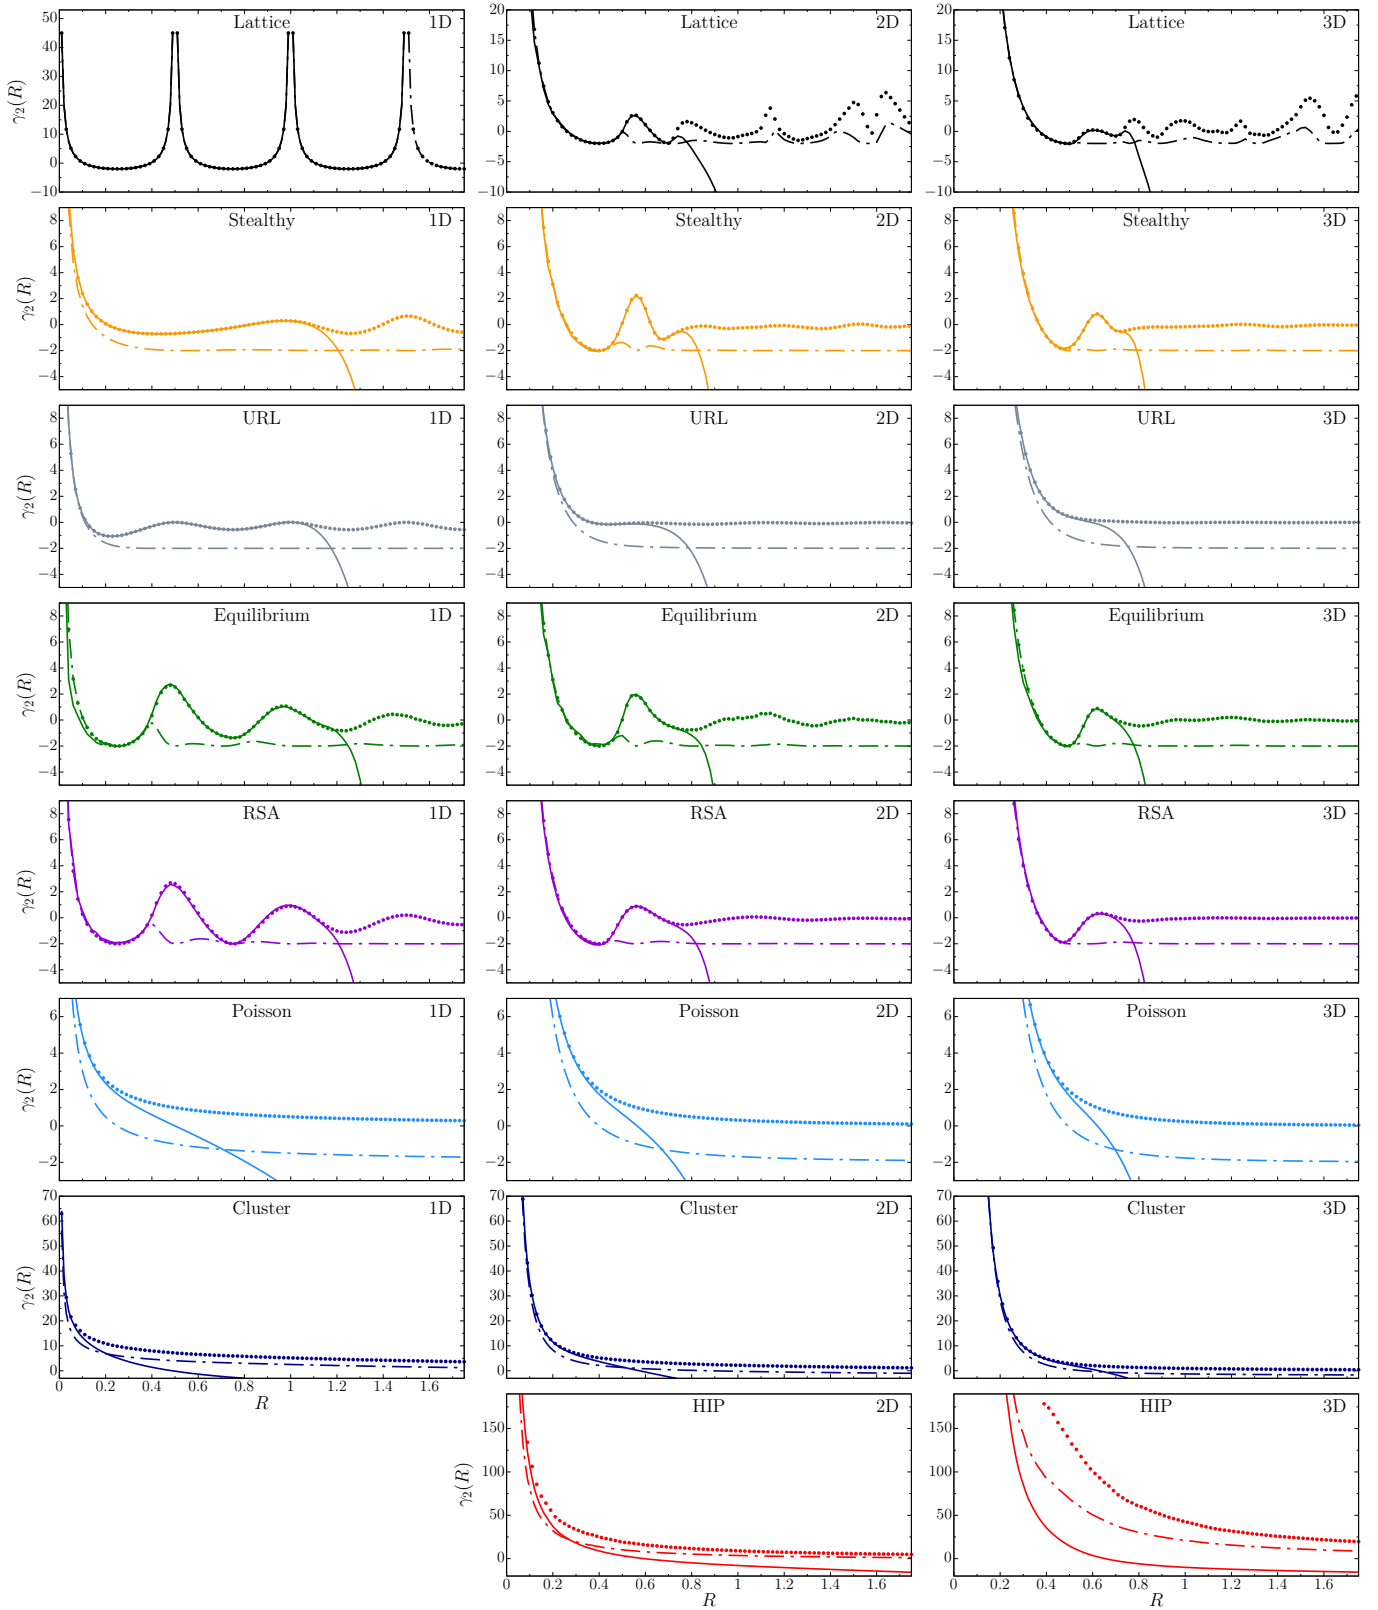

FIG. S2. Simulation results of the excess kurtosis  $\gamma_2(R)$  and their lower bounds, given in Eqs. (30) and (33) in the main article, for all models considered in this paper. The dotted lines represent our simulation results, and the solid and dash dotted lines are the bounds evaluated from (30) and (33), respectively. To evaluate these lower bounds, we employ the simulation results of  $\sigma^2(R)$  and  $\gamma_1(R)$ .

## B. Probability Density Function

In Sec. IIIB of the main article, it is shown that the probability distribution function  $P[N(R)]$  can be exactly expressed as a series expansion [see Eq. (40)], and their lower-order truncations can provide successive upper and lower bounds on  $P[N(R)]$ ; see Eqs. (41)–(44) in the main article. In Sec. IIIC, we show that these lower-order truncations can be exact for packings for sufficiently small values of  $R$ . Here, we compare our simulation results for  $P[N(R)]$  to the truncations of the series at the two- and three-body levels for all models considered in this work. Such comparisons validate our simulation results.

We begin with explicitly writing out the bounds in Eqs. (41)–(44) in the main article for  $N(R) = 0, 1, 2, 3$ . First, we consider  $P[N(R) = 0]$  which is bounded by

$$P[N(R) = 0] \leq \mathcal{A}_0(R), \quad (\text{S1})$$

$$P[N(R) = 0] \geq \mathcal{A}_0(R) - \mathcal{A}_1(R), \quad (\text{S2})$$

$$P[N(R) = 0] \leq \mathcal{A}_0(R) - \mathcal{A}_1(R) + \frac{1}{2}\mathcal{A}_2(R), \quad (\text{S3})$$

$$P[N(R) = 0] \geq \mathcal{A}_0(R) - \mathcal{A}_1(R) + \frac{1}{2}\mathcal{A}_2(R) - \frac{1}{6}\mathcal{A}_3(R). \quad (\text{S4})$$

Using Eqs. (21) and (22) from the main article, we can express  $\mathcal{A}_0(R)$  to  $\mathcal{A}_3(R)$  by  $\sigma^2(R)$  and  $C_3(R)$ :

$$\mathcal{A}_0(R) = 1, \quad (\text{S5})$$

$$\mathcal{A}_1(R) = \rho v_1(R), \quad (\text{S6})$$

$$\mathcal{A}_2(R) = \sigma^2(R) - \rho v_1(R)[1 - \rho v_1(R)], \quad (\text{S7})$$

$$\mathcal{A}_3(R) = C_3(R) - 3\sigma^2(R)[1 - \rho v_1(R)] + \rho v_1(R)[1 - \rho v_1(R)][2 - \rho v_1(R)]. \quad (\text{S8})$$

Thus, we obtain from Eqs. (S1)–(S4) the explicit bounds:

$$P[N(R) = 0] \leq 1, \quad (\text{S9})$$

$$P[N(R) = 0] \geq 1 - \rho v_1(R), \quad (\text{S10})$$

$$P[N(R) = 0] \leq [1 - \frac{1}{2}\rho v_1(R)][1 - \rho v_1(R)] + \frac{\sigma^2(R)}{2}, \quad (\text{S11})$$

$$P[N(R) = 0] \geq 1 - \rho v_1(R) - \frac{\rho v_1(R)}{6}[1 - \rho v_1(R)][5 - \rho v_1(R)] + \frac{1}{2}[2 - \rho v_1(R)]\sigma^2(R) - \frac{C_3(R)}{6}. \quad (\text{S12})$$

In the same way, we obtain from Eqs. (41)–(44) the following bounds on  $N(R) = 1$ :

$$P[N(R) = 1] \leq \mathcal{A}_1(R), \quad (\text{S13})$$

$$P[N(R) = 1] \geq \mathcal{A}_1(R) - \mathcal{A}_2(R), \quad (\text{S14})$$

$$P[N(R) = 1] \leq \mathcal{A}_1(R) - \mathcal{A}_2(R) + \frac{1}{2}\mathcal{A}_3(R), \quad (\text{S15})$$

$$P[N(R) = 1] \geq \mathcal{A}_1(R) - \mathcal{A}_2(R) + \frac{1}{2}\mathcal{A}_3(R) - \frac{1}{6}\mathcal{A}_4(R), \quad (\text{S16})$$

where the first three inequalities are explicitly given by:

$$P[N(R) = 1] \leq \rho v_1(R), \quad (\text{S17})$$

$$P[N(R) = 1] \geq 2\rho v_1(R) - [\rho v_1(R)]^2 - \sigma^2(R). \quad (\text{S18})$$

$$P[N(R) = 1] \leq \frac{1}{2}\rho v_1(R)[2 - \rho v_1(R)][3 - \rho v_1(R)] + \frac{1}{2}[-5 + 3\rho v_1(R)]\sigma^2(R) + \frac{1}{2}C_3(R). \quad (\text{S19})$$

Similar, we obtain the bounds on  $N(R) = 2$ :

$$P[N(R) = 2] \leq \frac{1}{2}\mathcal{A}_2(R), \quad (\text{S20})$$

$$P[N(R) = 2] \geq \frac{1}{2}\mathcal{A}_2(R) - \frac{1}{2}\mathcal{A}_3(R), \quad (\text{S21})$$

$$P[N(R) = 2] \leq \frac{1}{2}\mathcal{A}_2(R) - \frac{1}{2}\mathcal{A}_3(R) + \frac{1}{4}\mathcal{A}_4(R), \quad (\text{S22})$$

$$P[N(R) = 2] \geq \frac{1}{2}\mathcal{A}_2(R) - \frac{1}{2}\mathcal{A}_3(R) + \frac{1}{4}\mathcal{A}_4(R) - \frac{1}{12}\mathcal{A}_5(R), \quad (\text{S23})$$

where the first two inequalities are explicitly given by:

$$P[N(R) = 2] \leq \frac{\sigma^2(R)}{2} - \frac{\rho}{2}v_1(R)[1 - \rho v_1(R)], \quad (\text{S24})$$

$$P[N(R) = 2] \geq -\frac{\rho v_1(R)}{2}[1 - \rho v_1(R)][3 - \rho v_1(R)] + \frac{1}{2}[4 - 3\rho v_1(R)]\sigma^2(R) - \frac{1}{2}C_3(R). \quad (\text{S25})$$

Finally, we obtain the bounds on  $N(R) = 3$ :

$$P[N(R) = 3] \leq \frac{1}{6}\mathcal{A}_3(R), \quad (\text{S26})$$

$$P[N(R) = 3] \geq \frac{1}{6}\mathcal{A}_3(R) - \frac{1}{6}\mathcal{A}_4(R), \quad (\text{S27})$$

$$P[N(R) = 3] \leq \frac{1}{6}\mathcal{A}_3(R) - \frac{1}{6}\mathcal{A}_4(R) + \frac{1}{12}\mathcal{A}_5(R), \quad (\text{S28})$$

$$P[N(R) = 3] \geq \frac{1}{6}\mathcal{A}_3(R) - \frac{1}{6}\mathcal{A}_4(R) + \frac{1}{12}\mathcal{A}_5(R) - \frac{1}{36}\mathcal{A}_6(R), \quad (\text{S29})$$

where the first inequality is explicitly given by:

$$P[N(R) = 3] \leq \frac{\rho v_1(R)}{6}[1 - \rho v_1(R)][2 - \rho v_1(R)] - \frac{\sigma^2(R)}{2}[1 - \rho v_1(R)] + \frac{C_3(R)}{6}. \quad (\text{S30})$$

The aforementioned bounds become exact for hard spheres for certain values of  $R$  as explained in Sec. IIIC. Explicitly, the bounds of Eqs. (S10)–(S12), coincide with the expressions in Eqs. (50), (56) and (62); and so do Eqs. (S17)–(S19) with Eqs. (51), (57), and (63); as well as Eqs. (S24) and (S25) with Eqs. (58) and (64); and finally Eq. (S30) with Eq. (65).

In Figs. S3–S6, we compare our best upper and lower bounds to the simulation results.

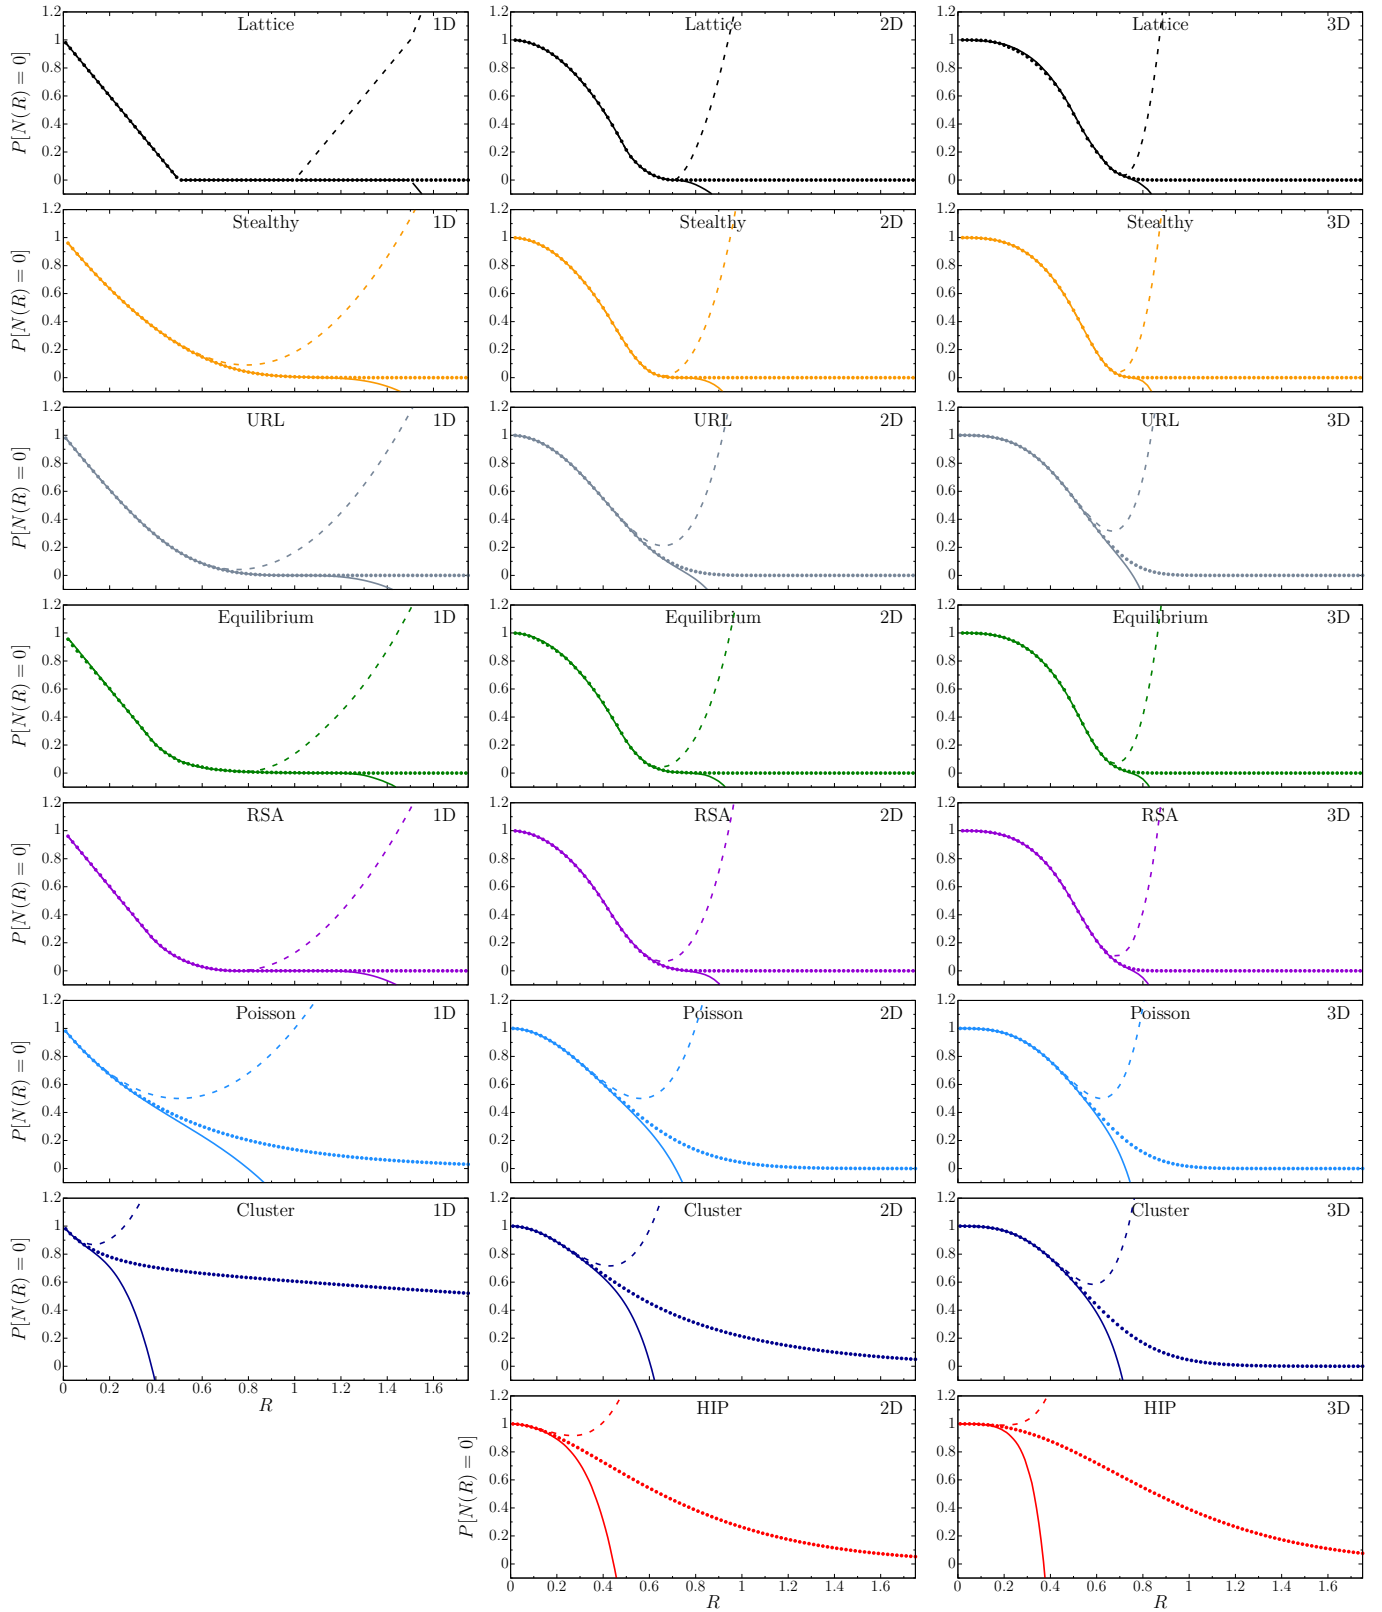

FIG. S3. Simulation results for the probability  $P[N(R)=0]$  of finding no points inside a window of radius  $R$  as a function of  $R$ , and corresponding bounds for all models considered in this work. The dotted lines represent our simulation results. The dashed and solid lines represent the upper and lower bounds from Eqs. (S11) and (S12), respectively. For packings, these bounds are exact for small values of  $R$ .

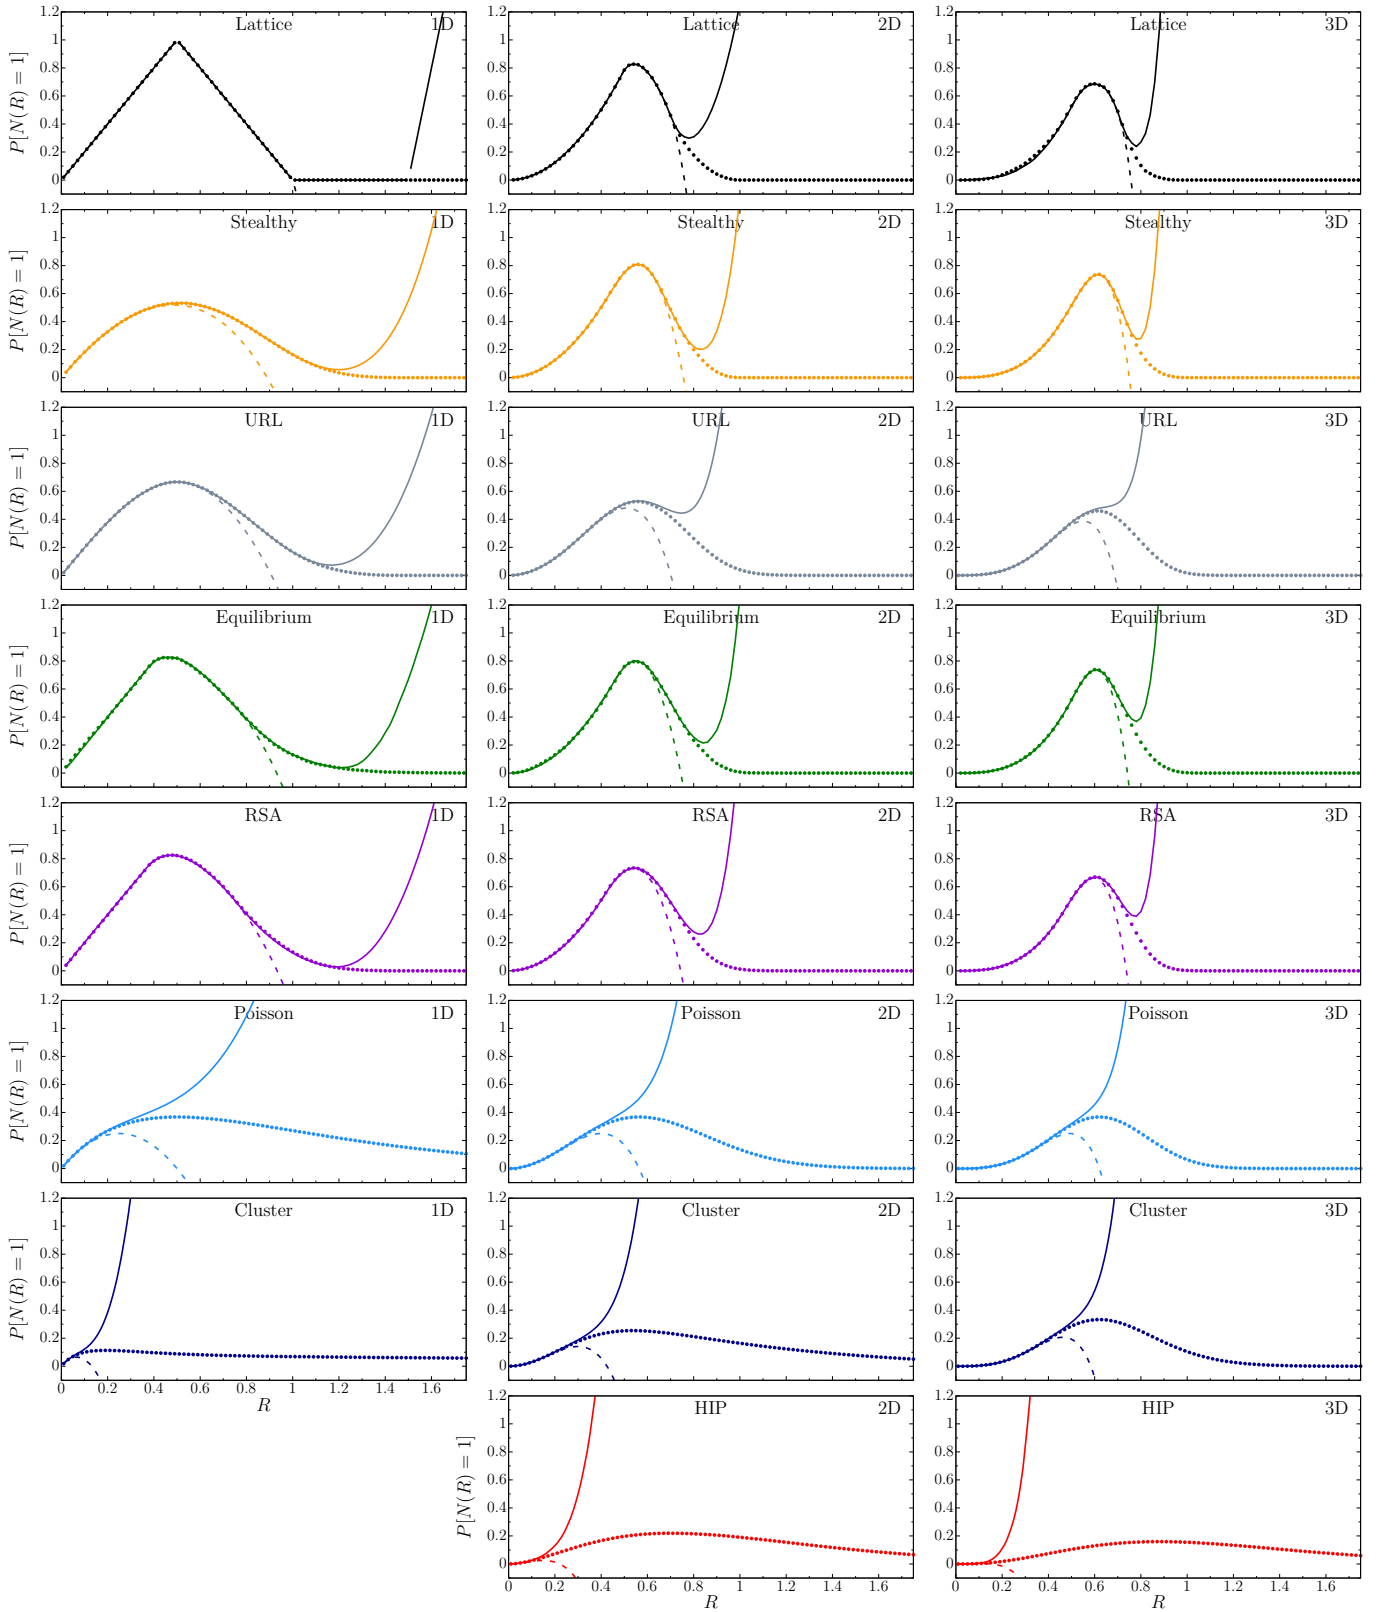

FIG. S4. Simulation results of the probability  $P[N(R) = 1]$  for finding a single point inside a window of radius  $R$  as a function of  $R$ , and corresponding bounds for all models considered in this work. The dotted lines represent our simulation results. The dashed and solid lines represent the lower and upper bounds from Eqs. (S18) and (S19), respectively. These bounds are also exact for packings for sufficiently small values of  $R$ .

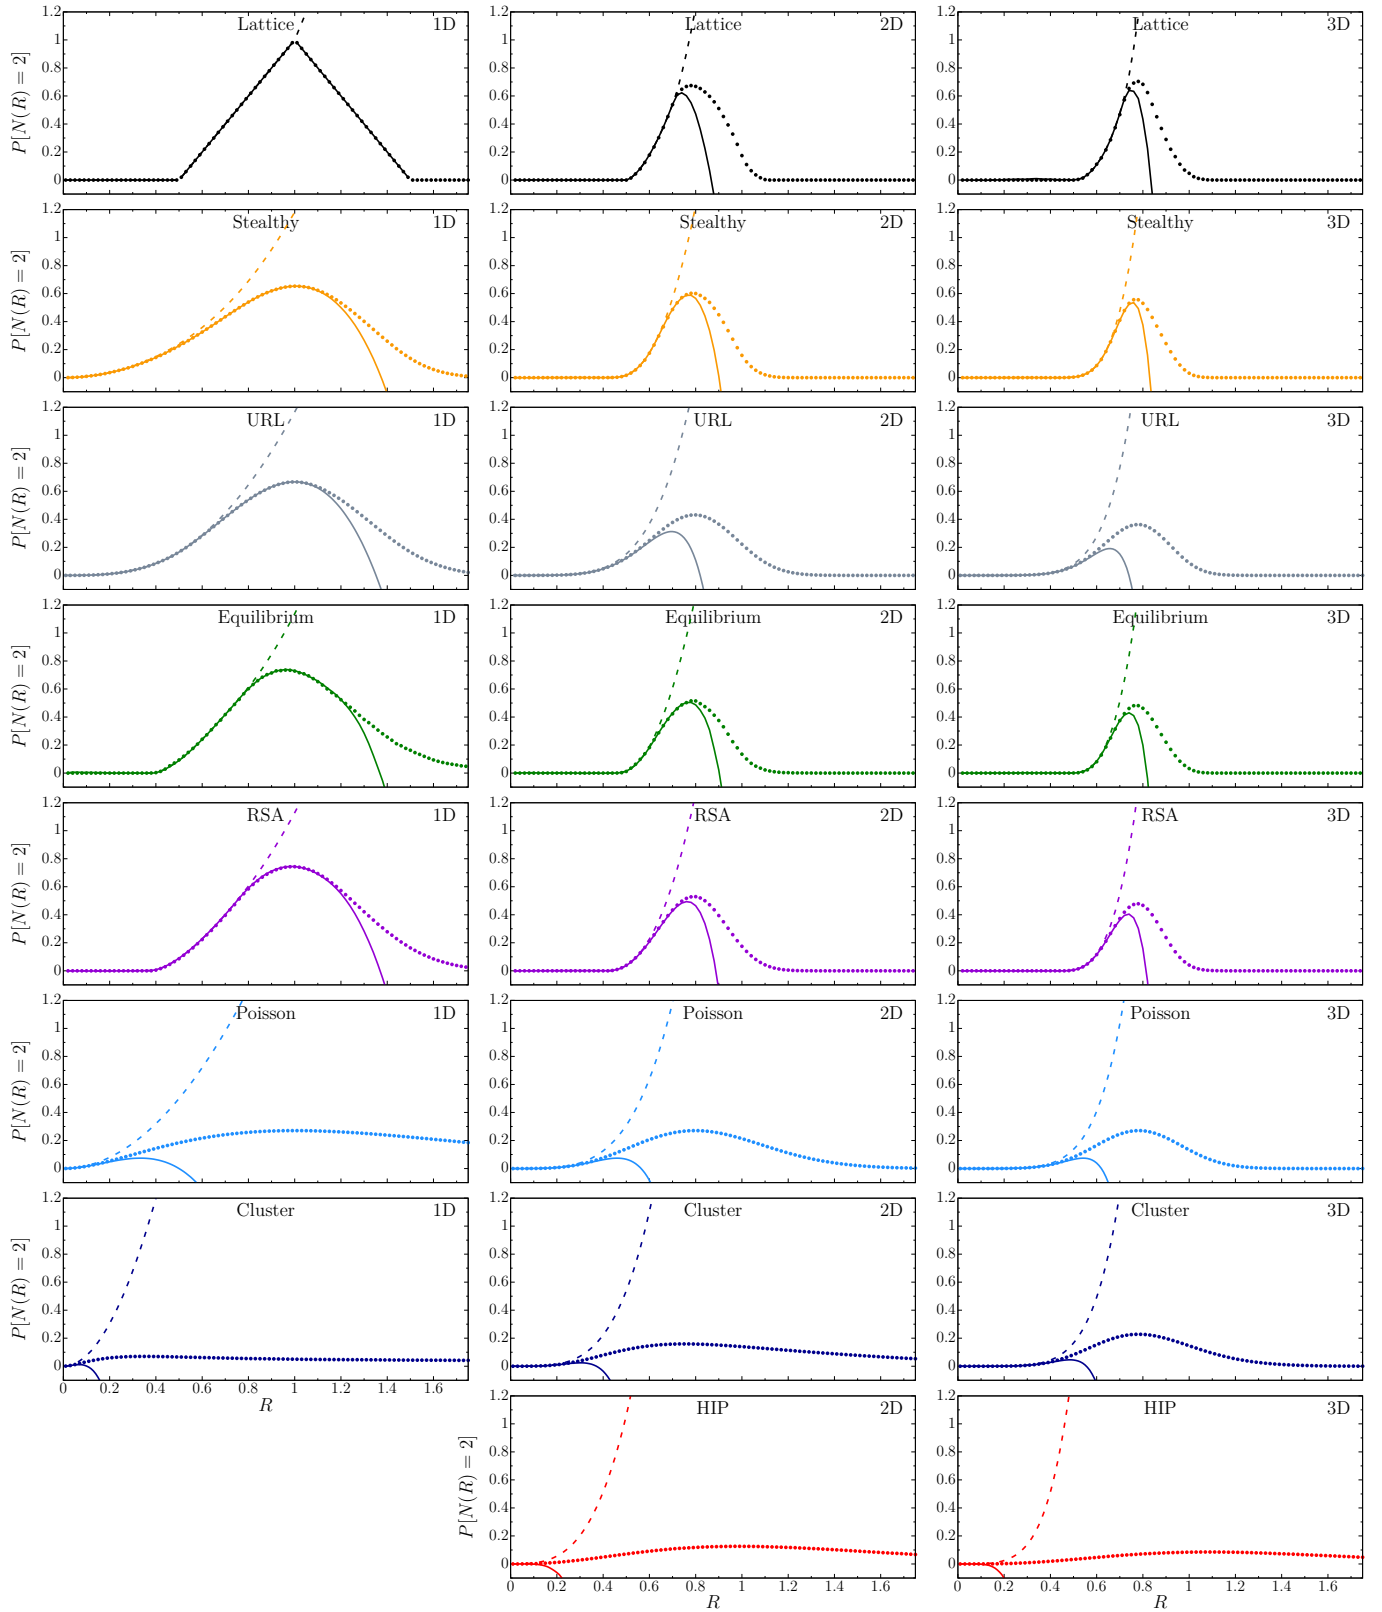

FIG. S5. Simulation results of the probability  $P[N(R)=2]$  for finding two points inside a window of radius  $R$  as a function of  $R$ , and corresponding bounds for all models considered in this work. The dotted lines represent our simulation results. The dashed and solid lines represent the upper and lower bounds from Eqs. (S24) and (S25), respectively. These bounds are also exact for packings for sufficiently small values of  $R$ .

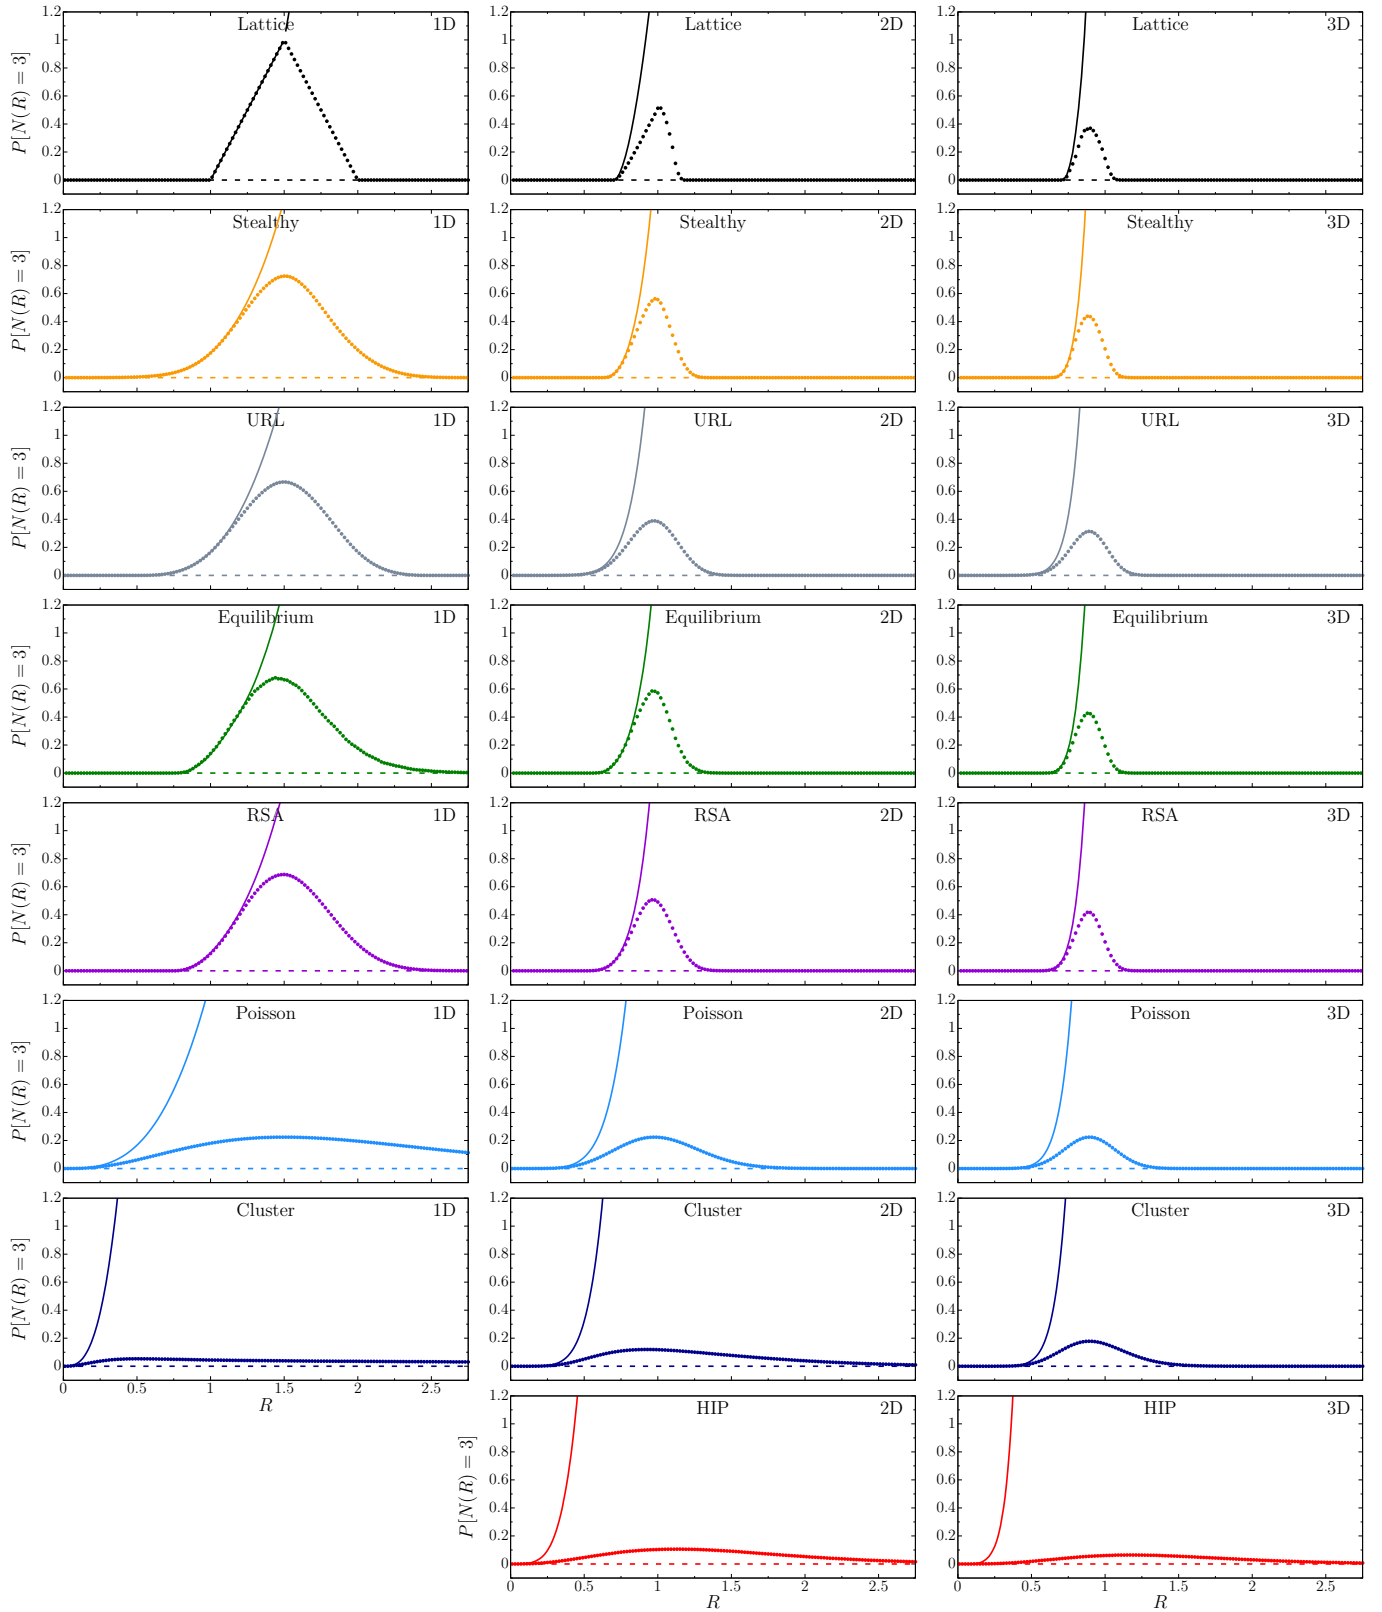

FIG. S6. Simulation results of the probability  $P[N(R) = 3]$  for finding three points inside a window of radius  $R$  as a function of  $R$ , and corresponding bounds for all models considered in this work. The dotted lines represent our simulation results. The solid line represents the upper bound from Eq. (S30). The bound is exact for packings for sufficiently small values of  $R$ . The dashed line shows the trivial lower bound  $P[N(R)] \geq 0$ .

## II. CONVERGENCE TO GAUSSIAN DISTRIBUTIONS

### A. Gaussian Distance Metrics

Here, we present the plots for two types of the Gaussian distance metrics that we discussed in the main article: one is the *Kullback-Leibler* divergence (also called the *relative entropy*), and another is the  $l_2(R)$  Gaussian distance metric that we proposed; see Eq. (81) of the main article. In the main article, we do not present the plots for the Kullback-Leibler divergence for the two reasons mentioned there. At a given window radius  $R$ , we define the Kullback-Leibler divergence from the normal distribution to  $P[N(R)]$  as

$$KL(R) \equiv \sum_{m=0}^{\infty} P[N(R) = m] \log \left( \frac{P[N(R) = m]}{P_{G(R)}(G(R) = m)} \right). \quad (\text{S31})$$

Figure S7 shows the Kullback-Leibler divergences for all models considered in this work.

Figure S8 shows the  $l_2(R)$  Gaussian distance metric for all models without cutting data (i.e.,  $R$  is up to  $R_{\max}$ ). It is interesting to note that for  $R > R_{\text{cut}}$ ,  $l_2(R)$  oscillates around  $o((N_{\text{window}} \times N_c)^{-1})$ , whereas  $KL(R)$  increases for large  $R$  due to statistical fluctuations in  $P[N(R)]$ , even in cases where  $KL(R) \gg (N_{\text{window}} \times N_c)^{-1}$ , for example, for the HIP and the Poisson cluster process in 3D. Such a difference makes it difficult to ascertain a CLT from the Kullback-Leibler divergence.

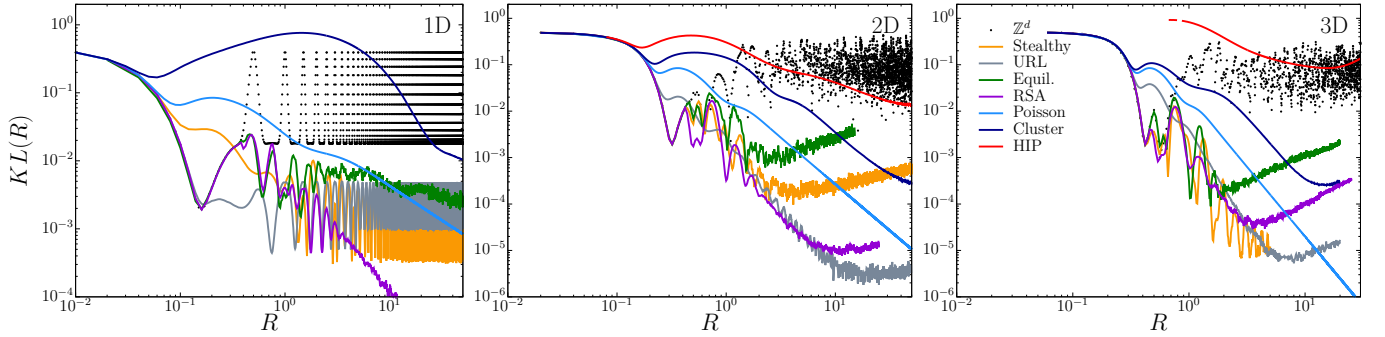

FIG. S7. Evaluation of the Kullback-Leibler divergence as a function of window radius  $R$  for all models considered in this work. This distance metric is evaluated from Eq. (S31).

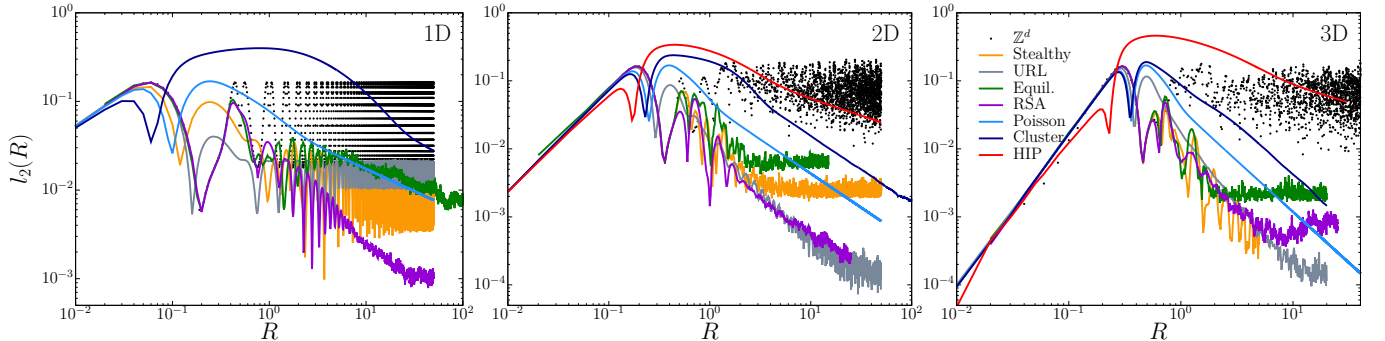

FIG. S8. Evaluation of the  $l_2(R)$  Gaussian distance metric as a function of window radius  $R$  for all models considered in this work. In contrast to the corresponding plot in the main article, we present the data beyond  $R_{\text{cut}}$ . For some models (e.g., 2D and 3D equilibrium packing, and 3D RSA), we see that  $l_2(R)$  no longer decreases for  $R > R_{\text{cut}}$  due to the finite number of sampling windows; see discussion in Sec. VI in the main article.

## B. Number Distribution Functions for 1D and 3D models

Here, we present the plots for the number distribution functions  $P[N(R)]$  for 1D and 3D models that were not included in the main article for brevity. The number distributions for the 1D nonhyperuniform and hyperuniform models are shown in Figs. S9 and S10, respectively. From these figures, we clearly see that while 1D nonhyperuniform models obey a CLT as  $R$  increases, 1D hyperuniform models do not obey a CLT.

The number distributions for the 3D nonhyperuniform and hyperuniform models are shown in Figs. S11 and S12, respectively. Visual inspection of Fig. S11 immediately reveals that all of the nonhyperuniform models, except 3D HIP, obey a CLT as  $R$  increases. However, a quantitative study via the Gaussian distance metric proves that the 3D HIP model also obeys a CLT. As shown in Fig. S12, all of the disordered hyperuniform models obeys a CLT, whereas the 3D simple cubic lattice does not.

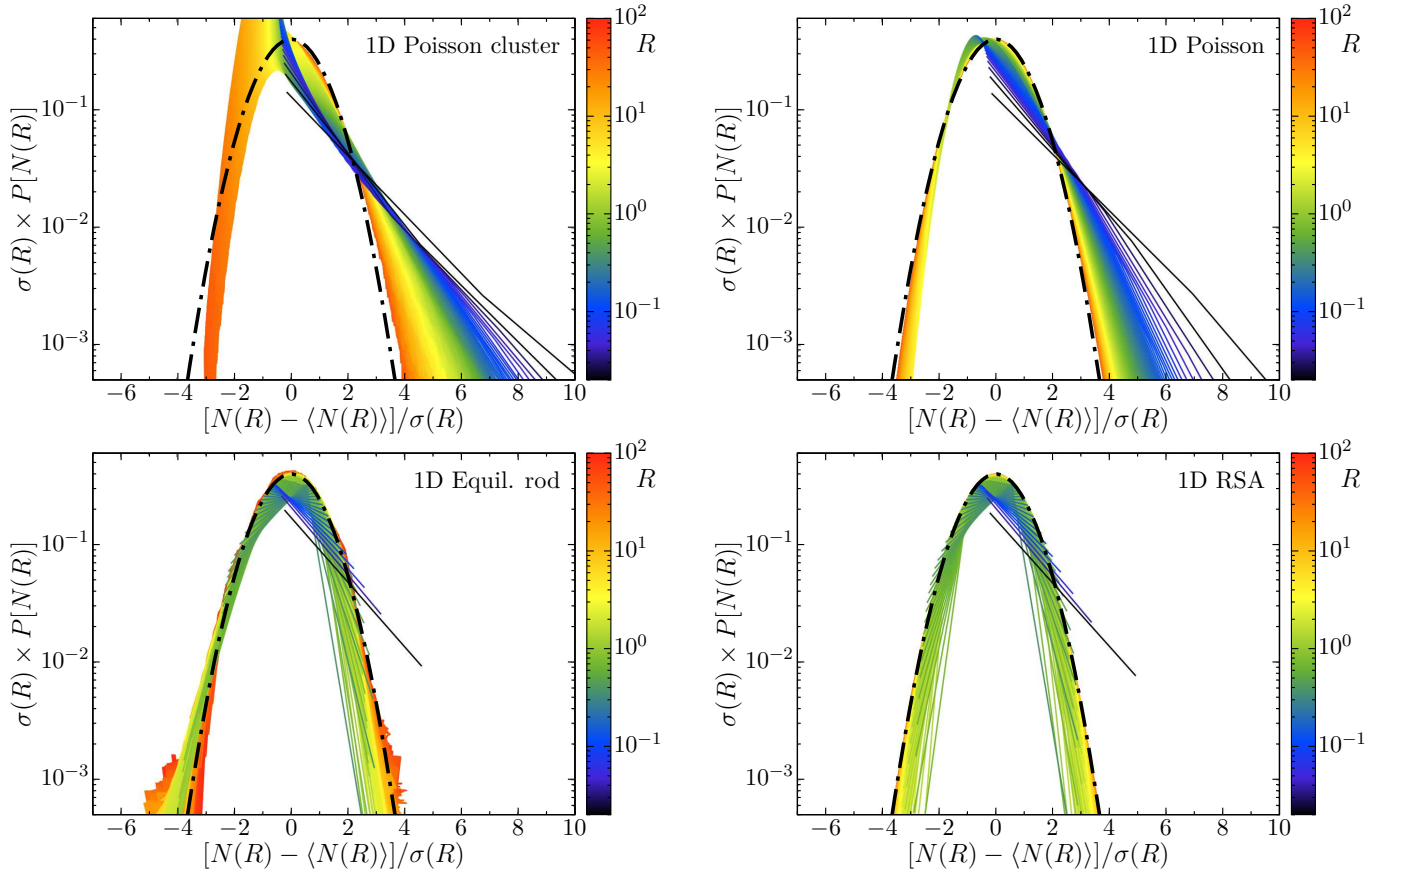

FIG. S9. Standardized probability distributions for the four 1D nonhyperuniform models (Poisson cluster process, Poisson point process, equilibrium hard rods, and saturated RSA) at various window radii; deepest blue color (darkest shade) corresponds to zero radius and the deep orange color corresponds to the largest considered radius. Note that Poisson cluster model has the largest value of  $S(0)$ , whereas the saturated RSA has the smallest one.

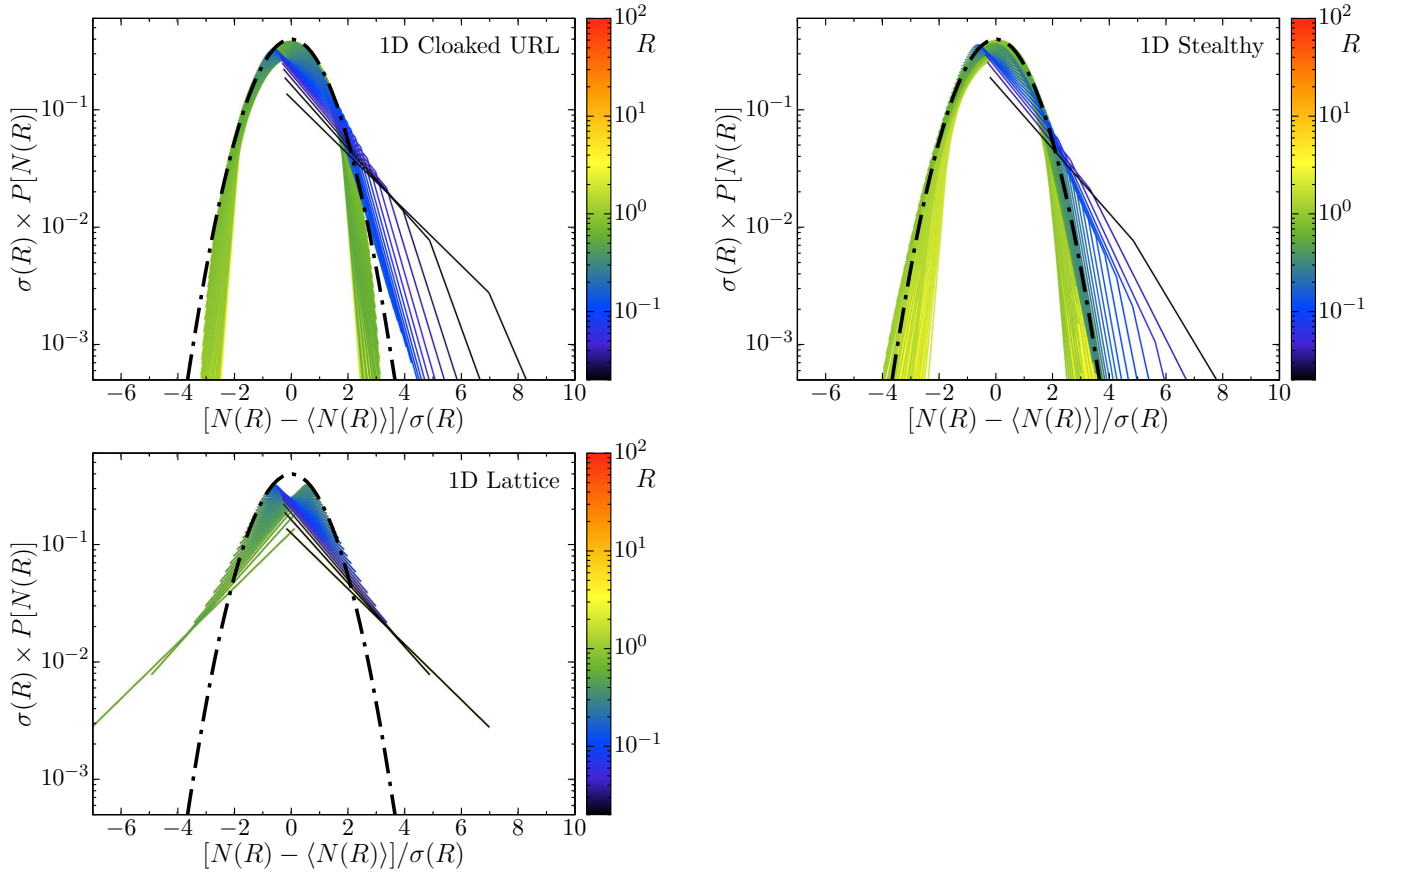

FIG. S10. Standardized probability distributions for the three 1D hyperuniform models (Cloaked URL model, entropically-favored stealthy hyperuniform model, and integer lattice) at various window radii; deepest blue color (darkest shade) corresponds to zero radius and the deep orange color corresponds to the largest considered radius.

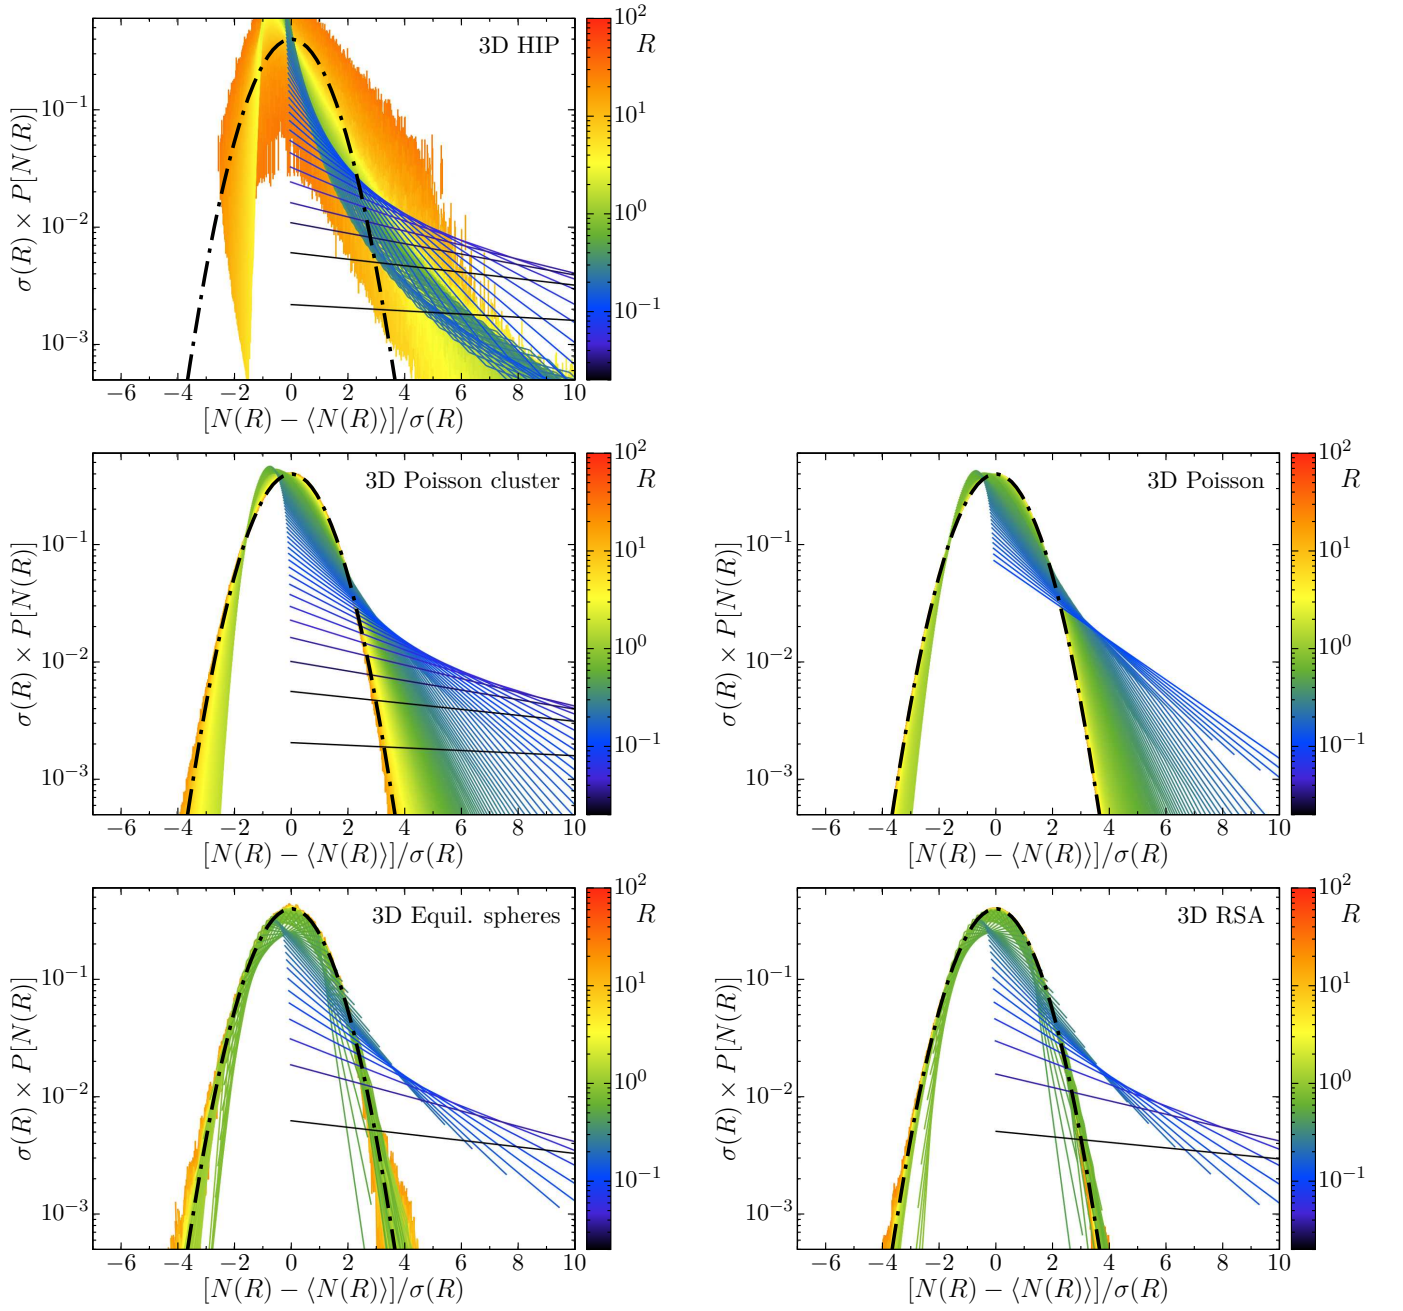

FIG. S11. Standardized probability distributions for the five 3D nonhyperuniform models (HIP model, Poisson cluster process, Poisson point process, equilibrium hard rods, and saturated RSA) at various window radii; deepest blue color (darkest shade) corresponds to zero radius and the deep orange color corresponds to the largest considered radius. Note that among nonhyperuniform models, except the HIP model, Poisson cluster model has the largest value of  $S(0)$ , whereas the saturated RSA has the smallest one.

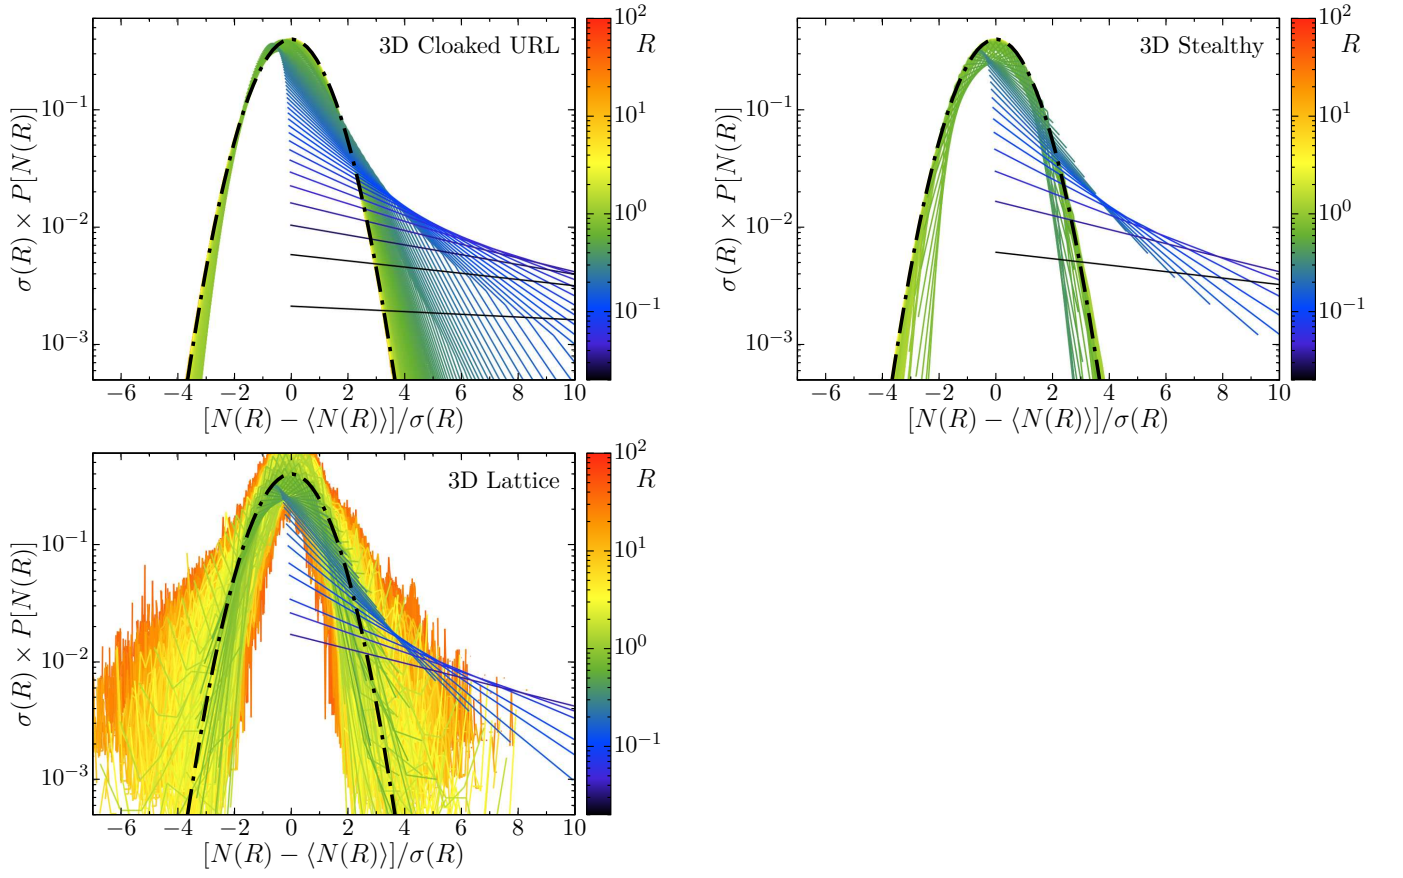

FIG. S12. Standardized probability distributions for the three 3D hyperuniform models, as per Fig. S10, at various window radii; deepest blue color (darkest shade) corresponds to zero radius and the deep orange color corresponds to the largest considered radius.

### C. Large- $R$ Scalings of Skewness, Excess Kurtosis, and Gaussian Distance Metric

The large- $R$  scaling behaviors of  $\gamma_1(R)$ ,  $\gamma_2(R)$  and  $l_2(R)$  are difficult to extract from the graphs shown in Figs. 2 and 5 in the main article for two reasons. First, the scaling regimes may only begin to manifest themselves at sufficiently large radii (e.g.,  $R > 10$ ), where robust numerical estimates are challenging due to the statistical and systematic errors. Another difficulty in this regard is the strong oscillations in  $\gamma_1(R)$ ,  $\gamma_2(R)$  and  $l_2(R)$  for some of the models. To robustly determine the large- $R$  behavior of these three quantities (and of their absolute values), we utilize the running-average (or cumulative-moving-average) procedure, which was previously used to study the asymptotic behavior of the number variance [1]. Specifically, we determine the large- $R$  behavior of a certain function  $f(R)$ , where  $f(R) = l_2(R)$ ,  $|\gamma_1(R)|$ , or  $|\gamma_2(R)|$  by first defining the running average  $\langle f \rangle_\beta(R)$ :

$$\langle f \rangle_\beta(R) \equiv \frac{1}{R^{\beta+1}} \int_0^R f(x) x^\beta dx, \quad (\text{S32})$$

where  $\beta$  is an sufficiently large exponent such that  $f(x)x^\beta = 0$  at  $x = 0$  and such that  $\langle f \rangle_\beta(R)$  captures the scaling behavior for large radii. Here, we use  $\beta = 5$ . The prefactor  $1/R^{\beta+1}$  in Eq. (S32) is chosen such that  $\langle f \rangle_\beta(R)$  has the same large- $R$  asymptotic behavior as  $f(R)$ . Figures S13–S15 show the running averages for our models in one, two, and three dimensions. Due to the strong oscillations in the excess kurtosis for 2D and 3D stealthy and URL processes described in the main article, a reliable estimate of the scaling is numerically challenging. For this reason, we do not include these special cases of the excess kurtosis in the numerical estimates depicted in Figs. S14 and S15.

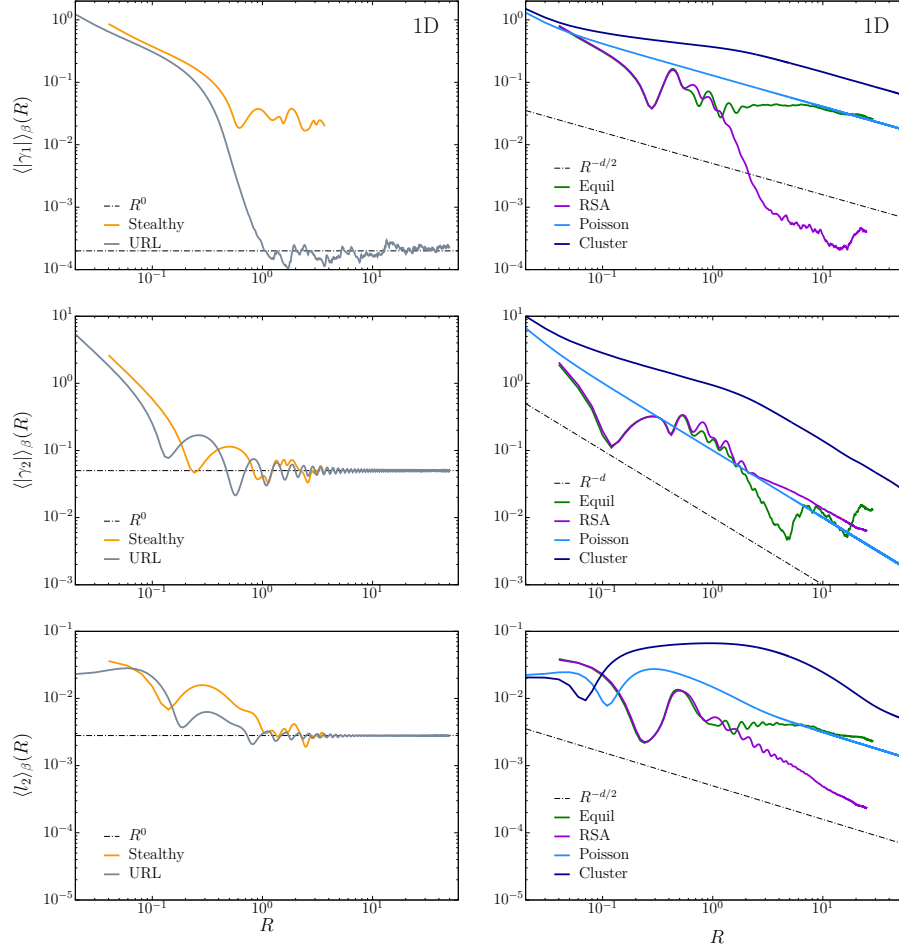

FIG. S13. Running averages, see Eq. (S32), of  $|\gamma_1(R)|$ ,  $|\gamma_2(R)|$ , and  $l_2(R)$  (top-bottom) for the disordered hyperuniform (left) and nonhyperuniform (right) 1D models considered in this work. For the nonhyperuniform models, the dash-dotted lines show the scalings predicted by the approximation of  $P[N(R)]$  with a gamma distribution. For the hyperuniform models, the dash-dotted lines are constant because in one dimension class I hyperuniform models cannot obey a CLT.

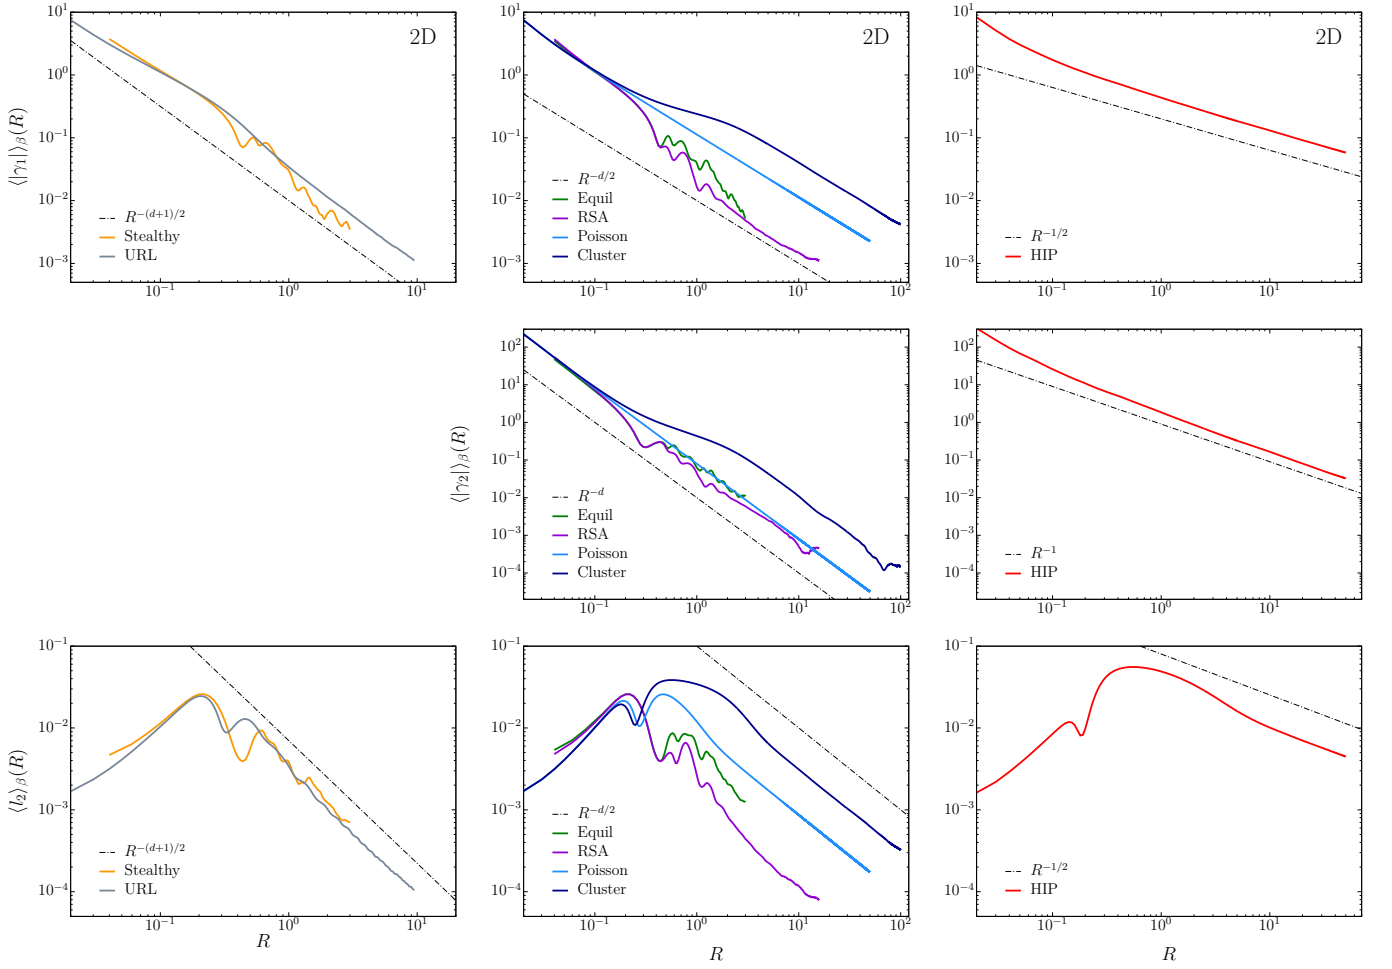

FIG. S14. Running averages, see Eq. (S32), of  $|\gamma_1(R)|$ ,  $|\gamma_2(R)|$ , and  $l_2(R)$  (top–bottom) for the disordered hyperuniform (left), nonhyperuniform (center), and antihyperuniform (right) 2D models considered in this work. The dash-dotted lines show the scalings predicted by the approximation of  $P[N(R)]$  with a gamma distribution. As explained in the text, we do not include the plot for  $|\gamma_2(R)|$  of the hyperuniform models because of the numerical challenges due to the strong oscillations.

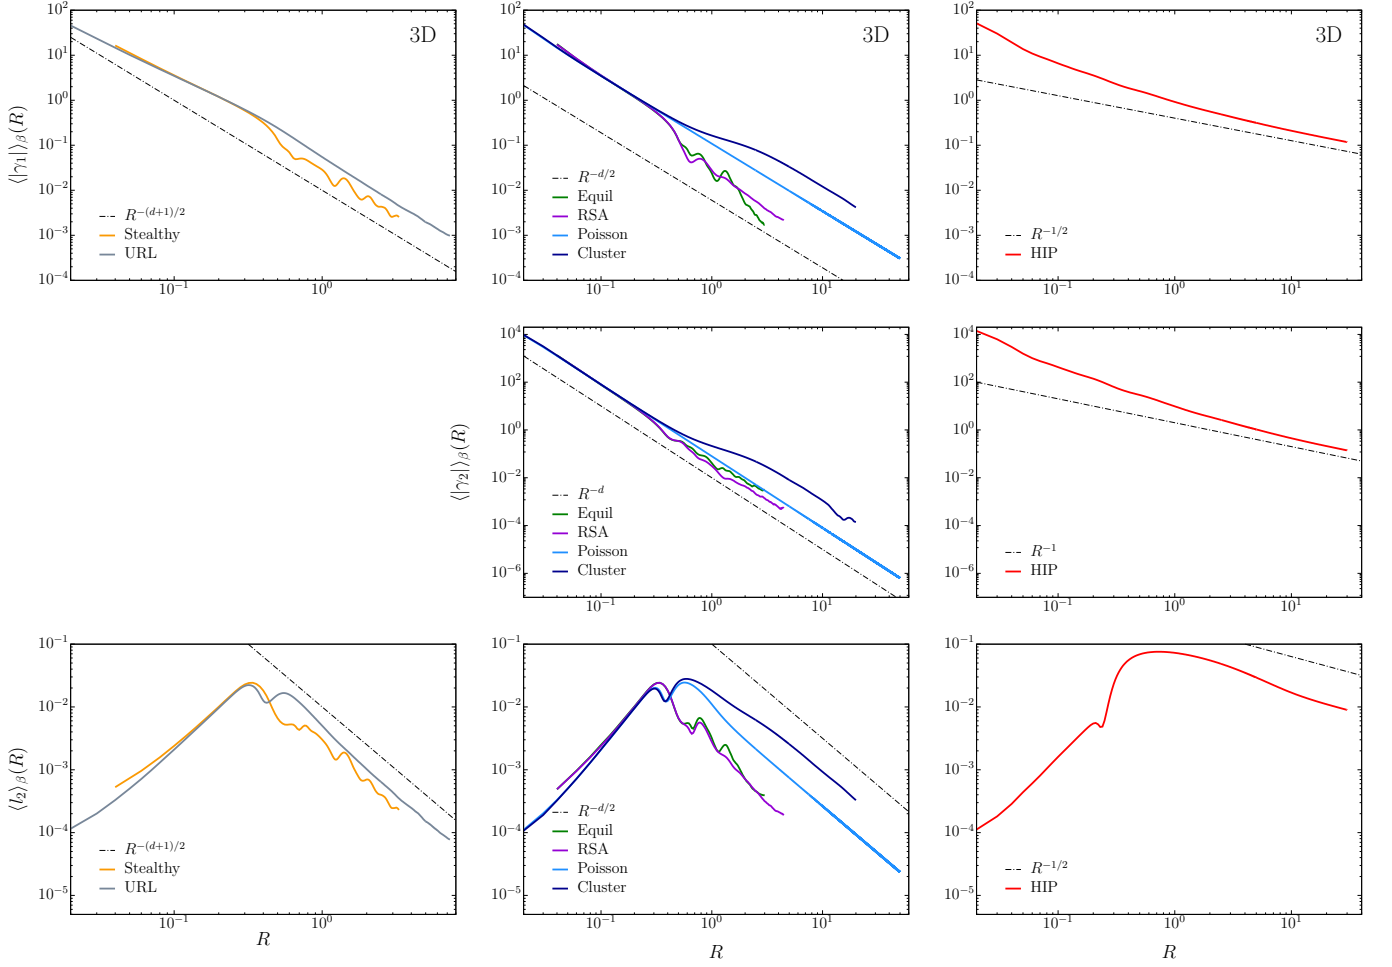

FIG. S15. Running averages, see Eq. (S32), of  $|\gamma_1(R)|$ ,  $|\gamma_2(R)|$ , and  $l_2(R)$  (top–bottom) for the disordered hyperuniform (left), nonhyperuniform (center), and antihyperuniform (right) 3D models considered in this work. The dash-dotted lines show the scalings predicted by the approximation of  $P[N(R)]$  with a gamma distribution. As explained in the text, we do not include the plot for  $|\gamma_2(R)|$  of the hyperuniform models because of the numerical challenges due to the strong oscillations.

### III. GAMMA-DISTRIBUTION APPROXIMATION

Here, we demonstrate that the gamma distribution provides a good approximation to the number distribution  $P[N(R)]$  for all models that obey a CLT for intermediate values of  $R$ . Figures S16 and S17 compare the probability distributions  $P[N(R)]$  at  $R = 10.0$  to their gamma-distribution approximations for 1D nonhyperuniform and hyperuniform models, respectively. The gamma distribution shows good agreement with  $P[N(R)]$  for 1D nonhyperuniform models that obey a CLT. However, for 1D hyperuniform models that do not obey a CLT, the gamma distribution cannot provide a good approximation, as expected from their bounded supports.

Figures S18 and S19 compare  $P[N(R)]$  and their corresponding gamma-distribution approximations for 2D nonhyperuniform and hyperuniform models, respectively, for  $R = 5.0$ . These figures demonstrate that for all models, except for the square lattice, the gamma distribution provides a good approximation to  $P[N(R)]$ . As noted in the main article, the square lattice does not obey a CLT.

Figures S20 and S21 compare  $P[N(R)]$  and their corresponding gamma-distribution approximations for 3D nonhyperuniform and hyperuniform models, respectively, for  $R = 3.0$ . These figures demonstrate that for all models, except for the simple cubic lattice, the gamma distribution provides a good approximation to  $P[N(R)]$ . As noted in the main article, the simple cubic lattice does not obey a CLT.

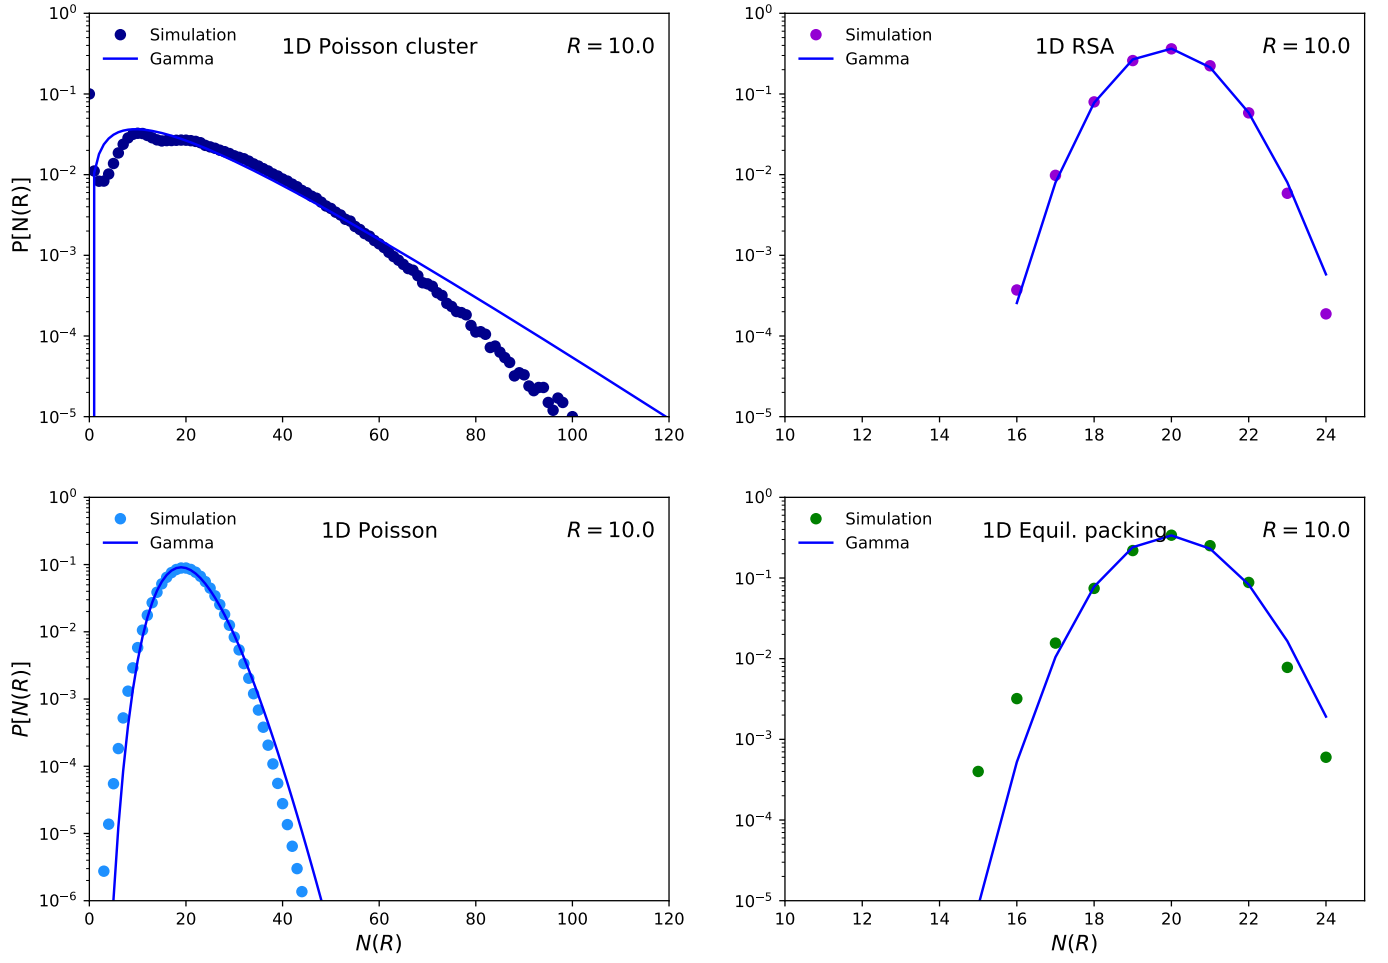

FIG. S16. Semi-logarithmic plots of the probability distributions  $P[N(R)]$  for 1D nonhyperuniform models (Poisson cluster, Poisson, RSA, and equilibrium packing) at  $R = 10.0$  and their gamma-distribution approximations.

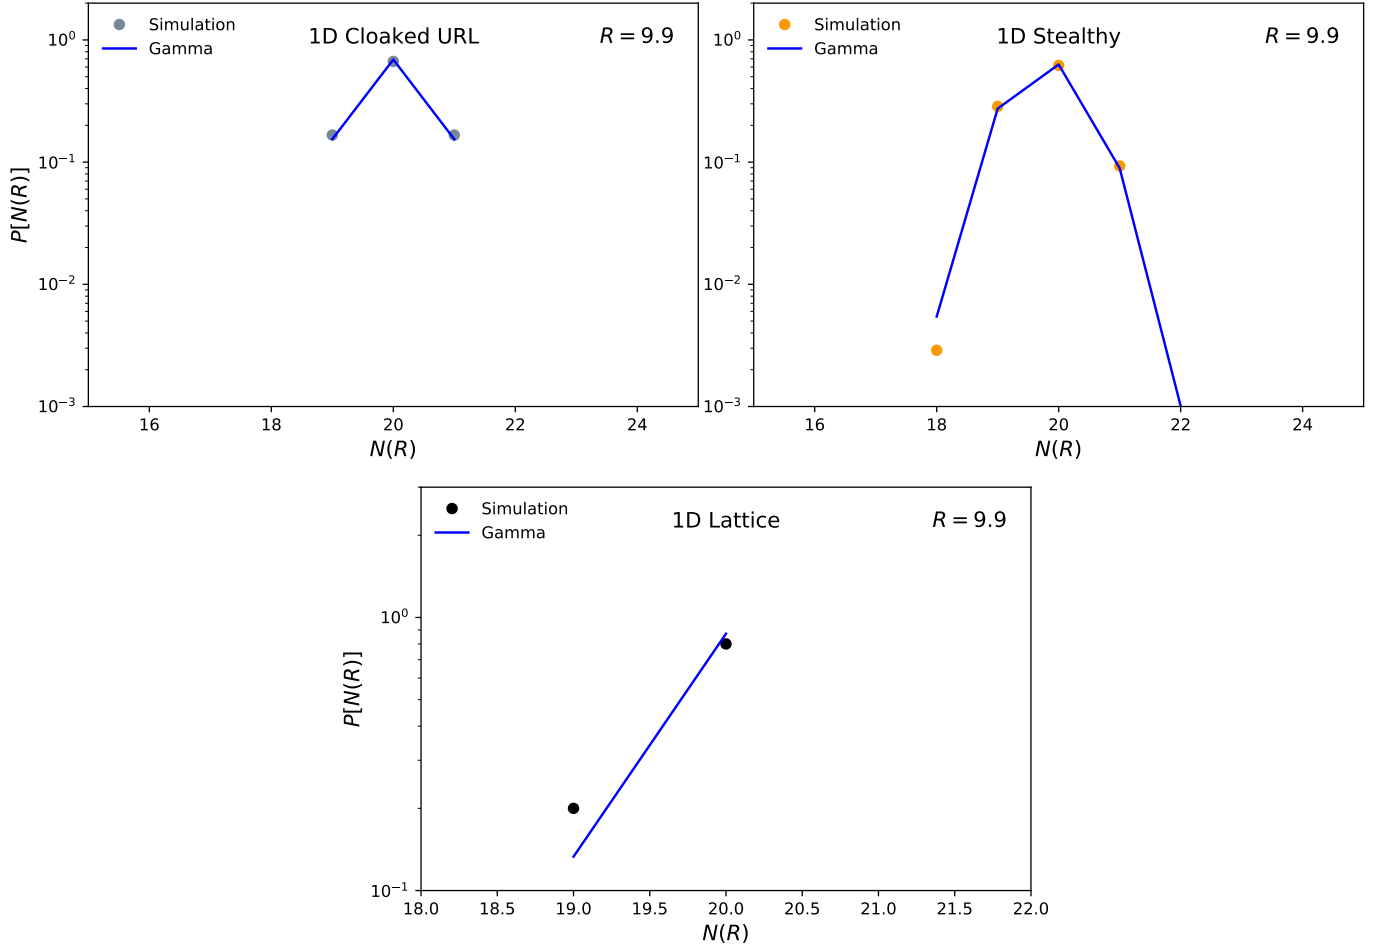

FIG. S17. Semi-logarithmic plots of the probability distributions  $P[N(R)]$  for 1D hyperuniform models (cloaked URL, stealthy hyperuniform, and lattice) at  $R = 10.0$  and their gamma-distribution approximations.

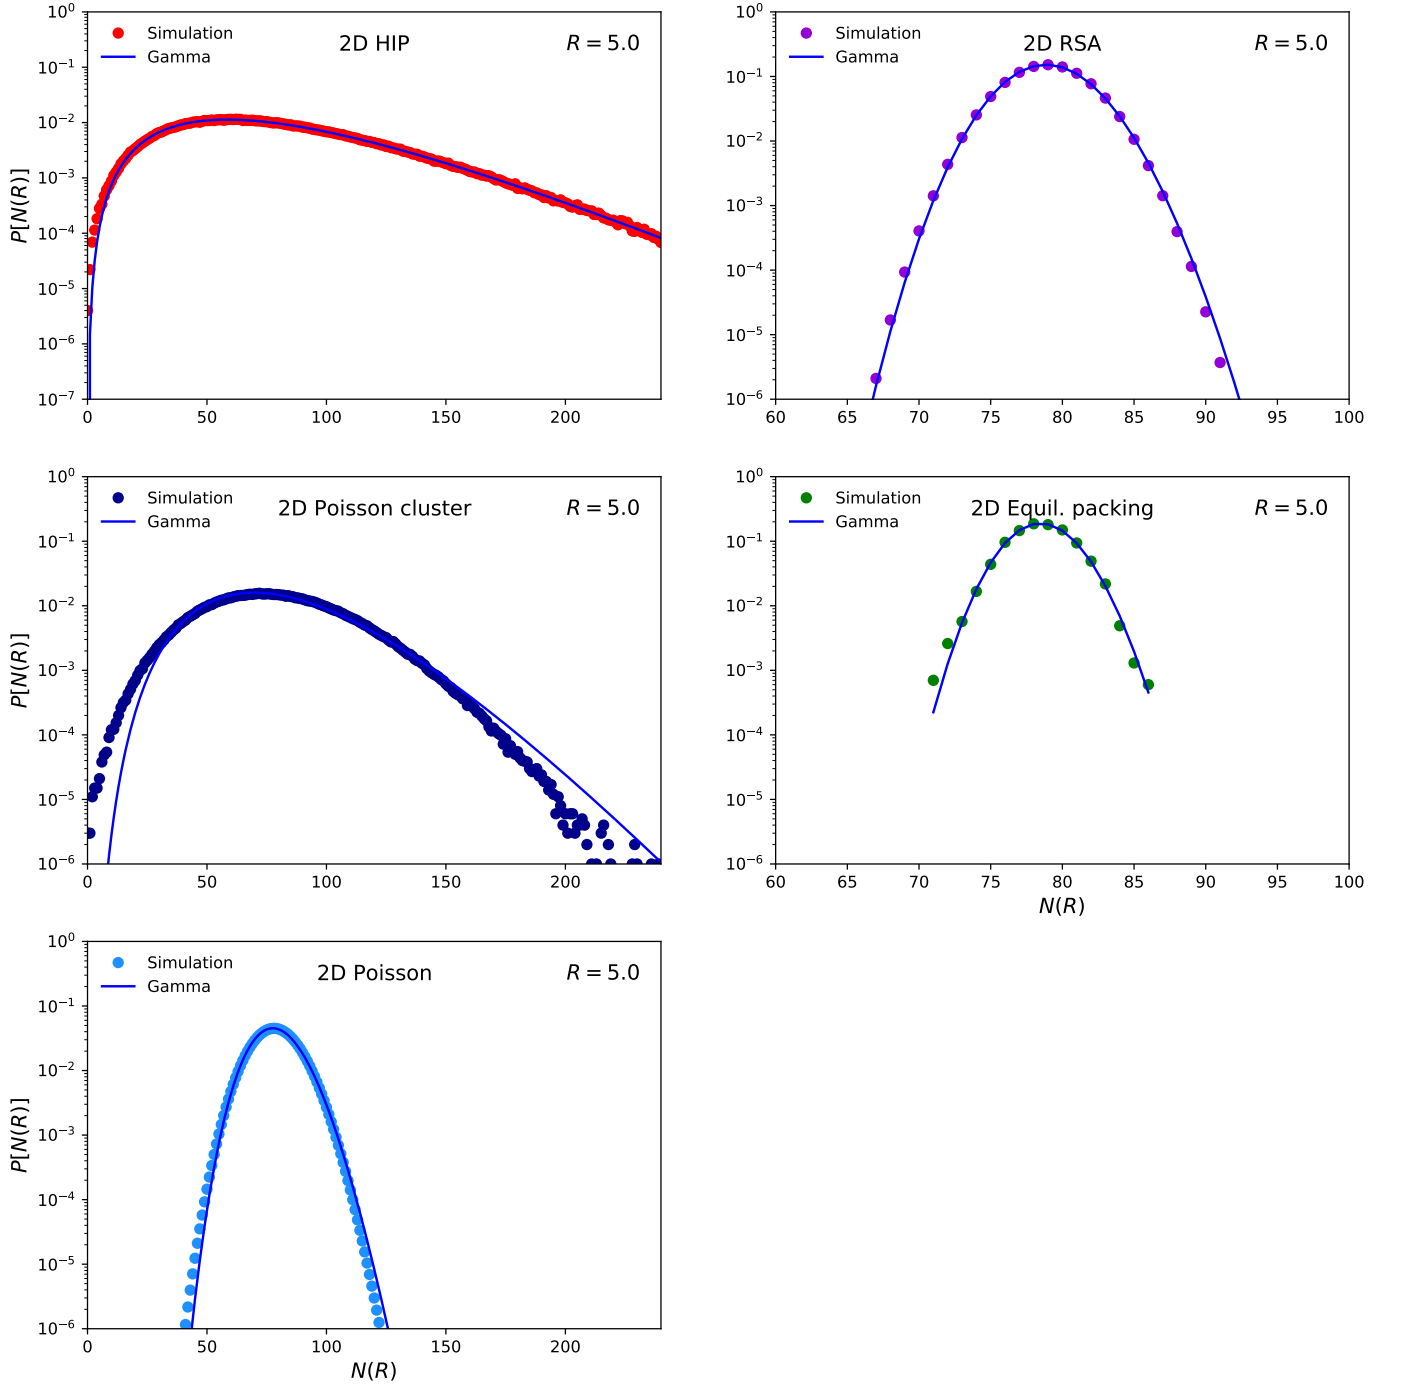

FIG. S18. Semi-logarithmic plots of the probability distributions  $P[N(R)]$  for 2D nonhyperuniform models (HIP, Poisson cluster, Poisson, RSA, and equilibrium packing) at  $R = 5.0$  and their gamma-distribution approximations.

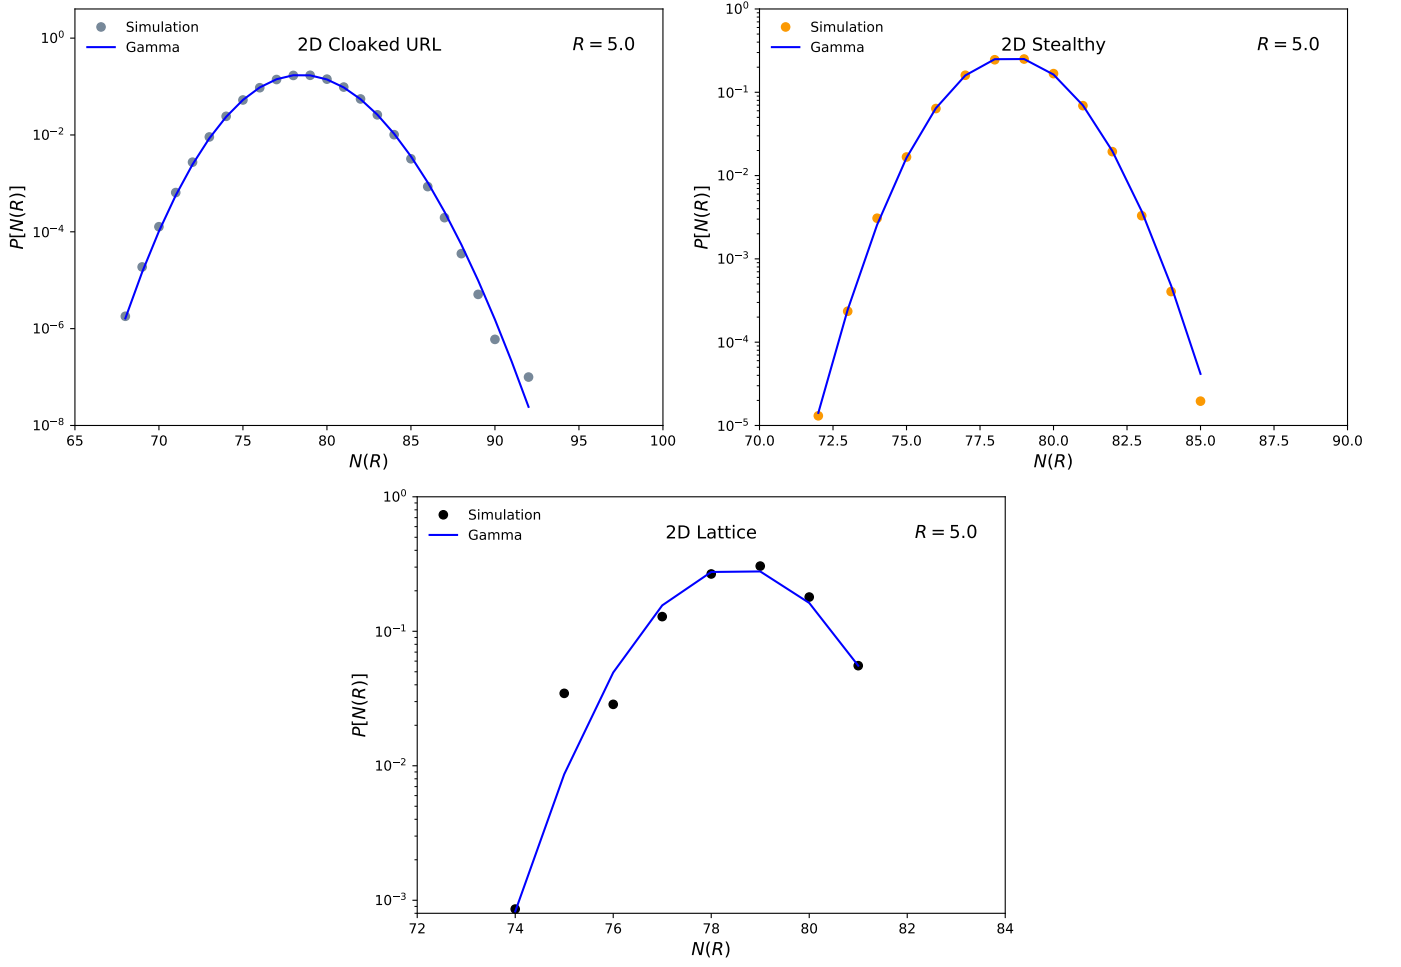

FIG. S19. Semi-logarithmic plots of the probability distributions  $P[N(R)]$  for 2D hyperuniform models (cloaked URL, stealthy hyperuniform, and lattice) at  $R = 5.0$  and their gamma-distribution approximations.

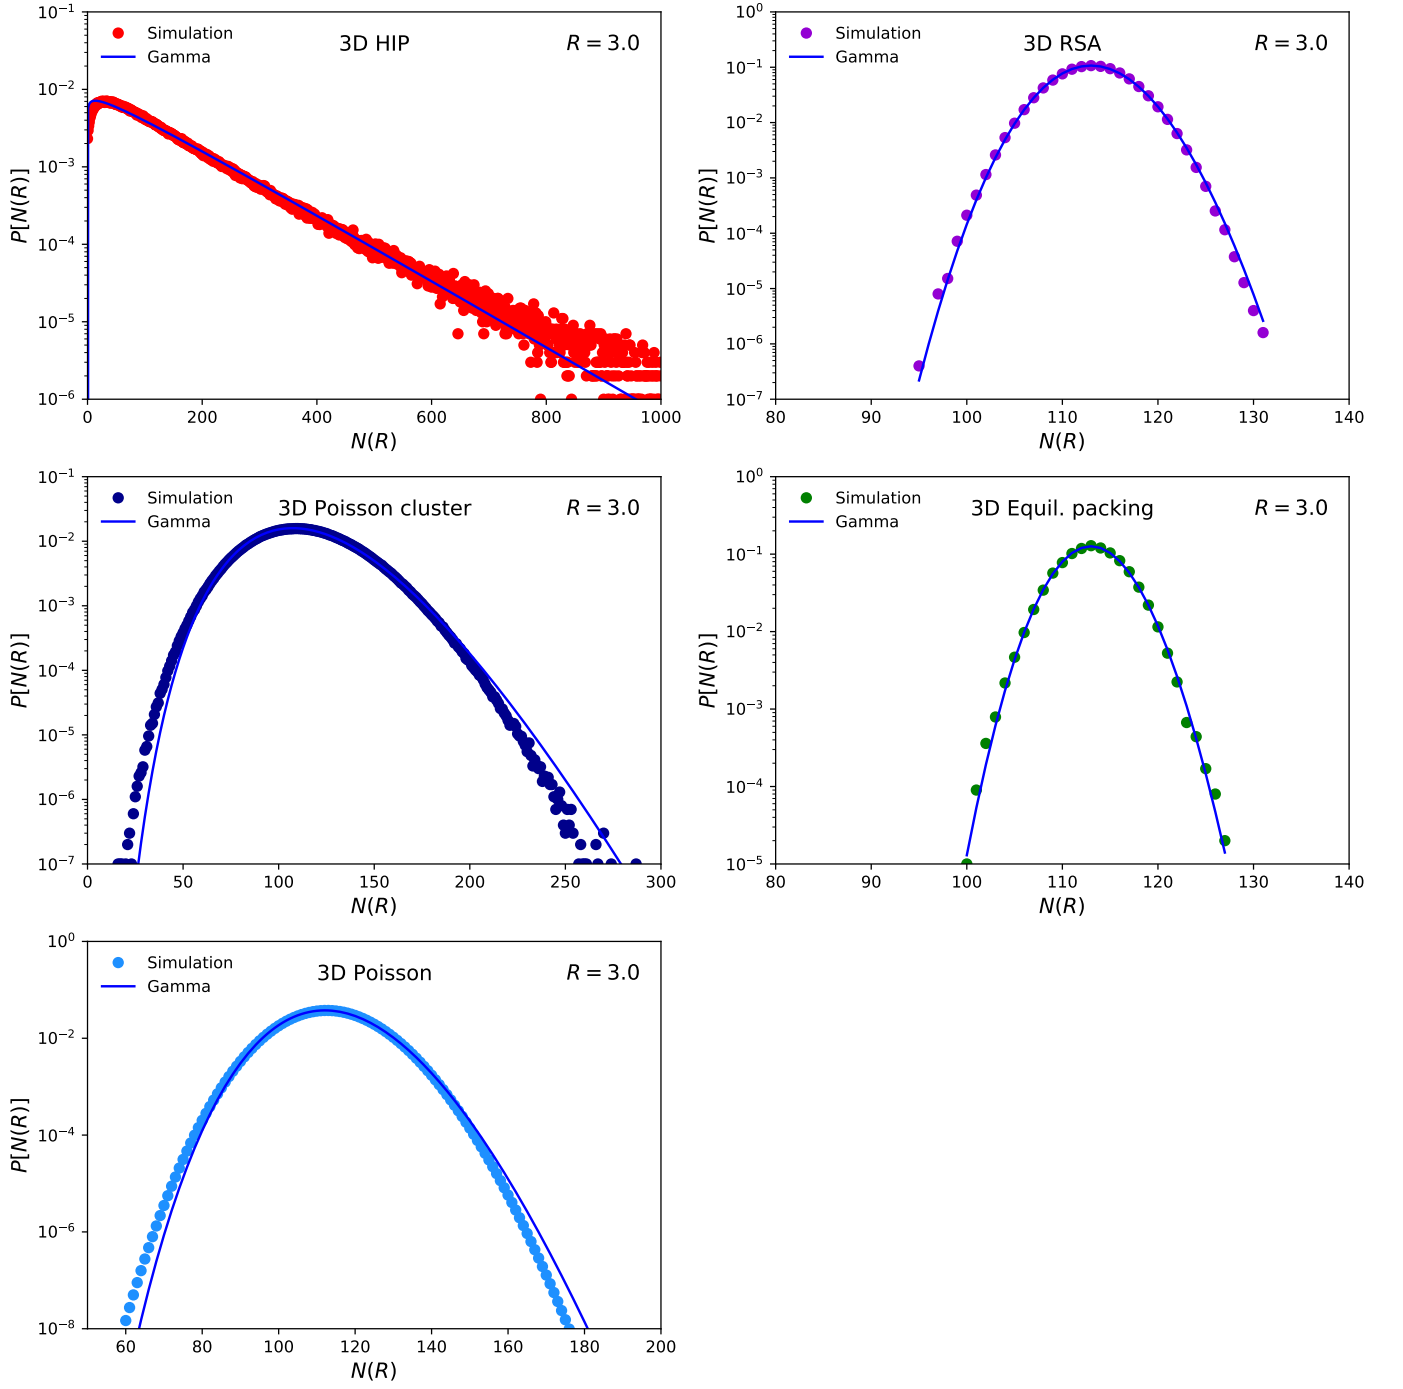

FIG. S20. Semi-logarithmic plots of the probability distributions  $P[N(R)]$  for 3D nonhyperuniform models (HIP, Poisson cluster, Poisson, RSA, and equilibrium packing) at  $R = 3.0$  and their gamma-distribution approximations.

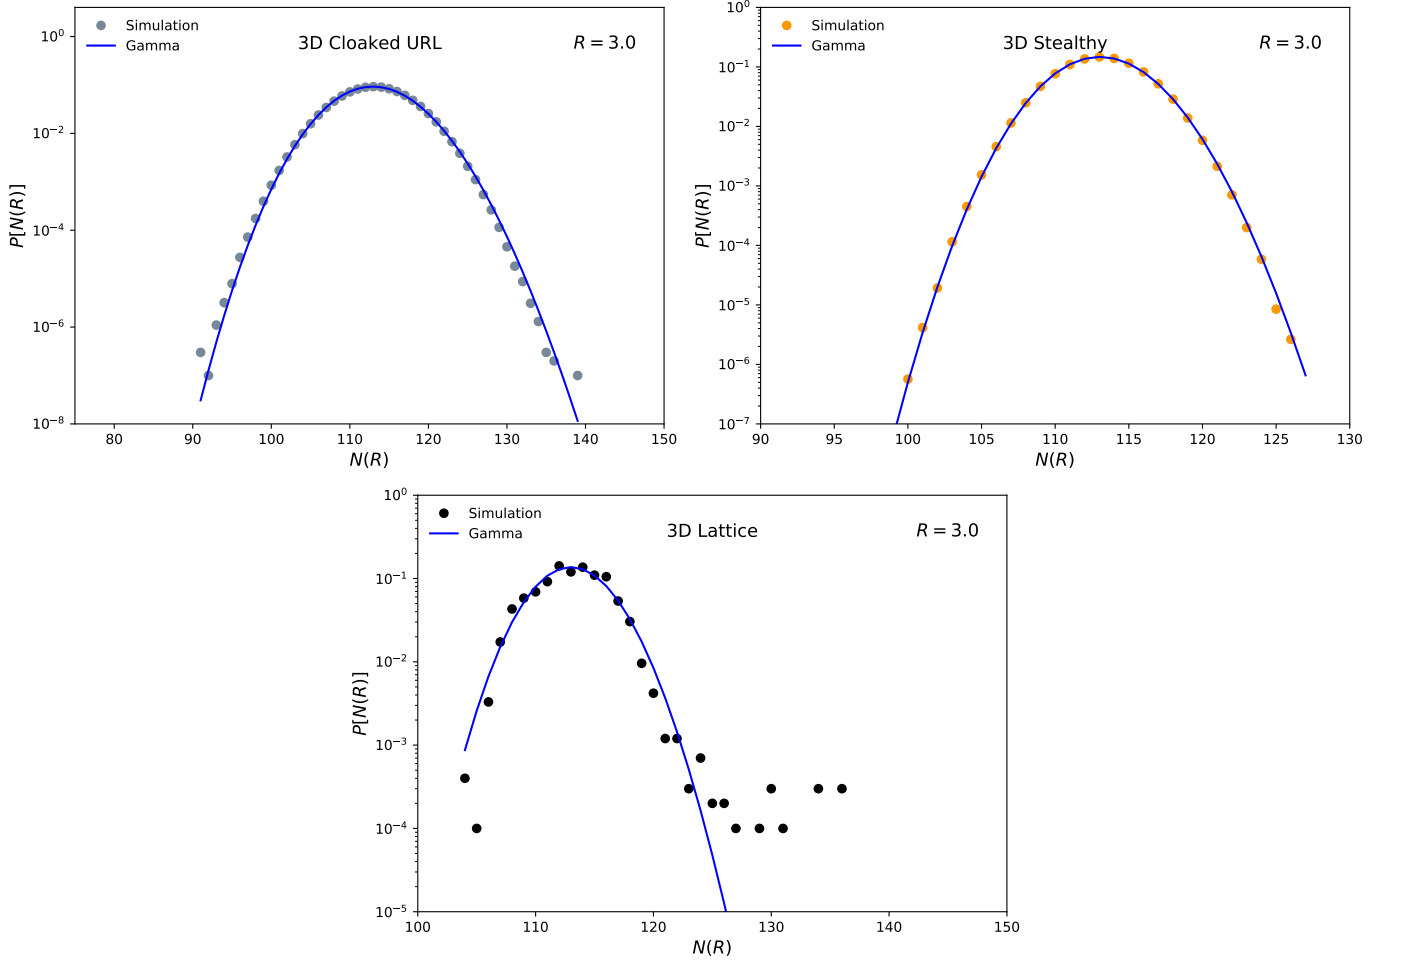

FIG. S21. Semi-logarithmic plots of the probability distributions  $P[N(R)]$  for 3D hyperuniform models (cloaked URL, stealthy hyperuniform, and lattice) at  $R = 3.0$  and their gamma-distribution approximations.

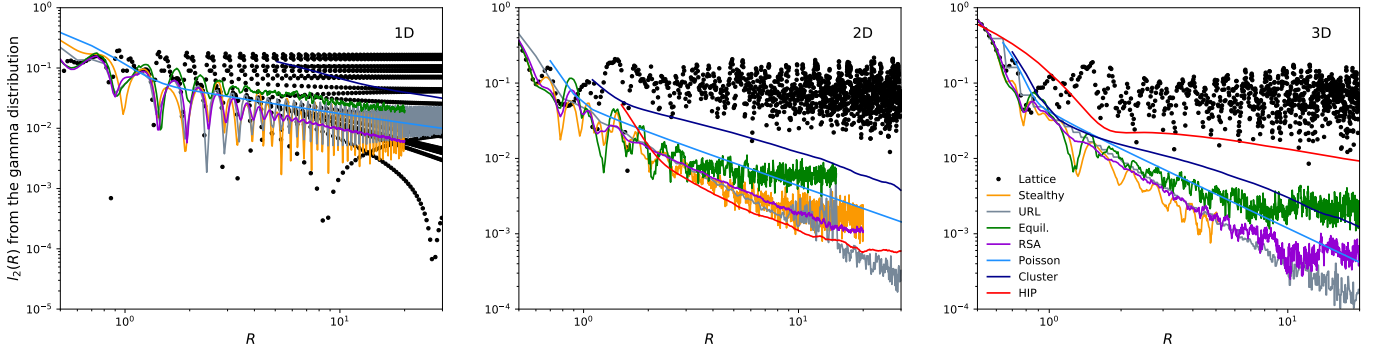

FIG. S22. Log-log plots of the  $l_2(R)$  distance metric of the number distributions  $P[N(R)]$  from their gamma-distribution approximation as a function of window radius  $R$  for all models considered in this work.

In order to quantitatively measure how accurately the gamma distribution approximates  $P[N(R)]$ , we evaluate a type of  $l_2$  distance metric (see Fig. S22) but where the reference distribution is the gamma distribution. For all models, except those that do not obey a CLT,  $l_2(R)$  decreases with  $R$ , proving that the gamma distribution provides a good approximation to  $P[N(R)]$ .

We numerically obtain the large- $R$  scaling of  $l_2(R)$  described in Table II of the main article; see Fig. S23. To do so, for each model obeying a CLT, we first obtain the gamma-distribution approximation from  $\langle N(R) \rangle$  and  $\sigma^2(R)$  at a given value of  $R$ , and then evaluate the  $l_2(R)$  Gaussian distance metric of the approximation. As we noted in the main article, the obtained scaling of  $l_2(R)$  is identical to that of the skewness  $\gamma_1(R)$  for the corresponding model.

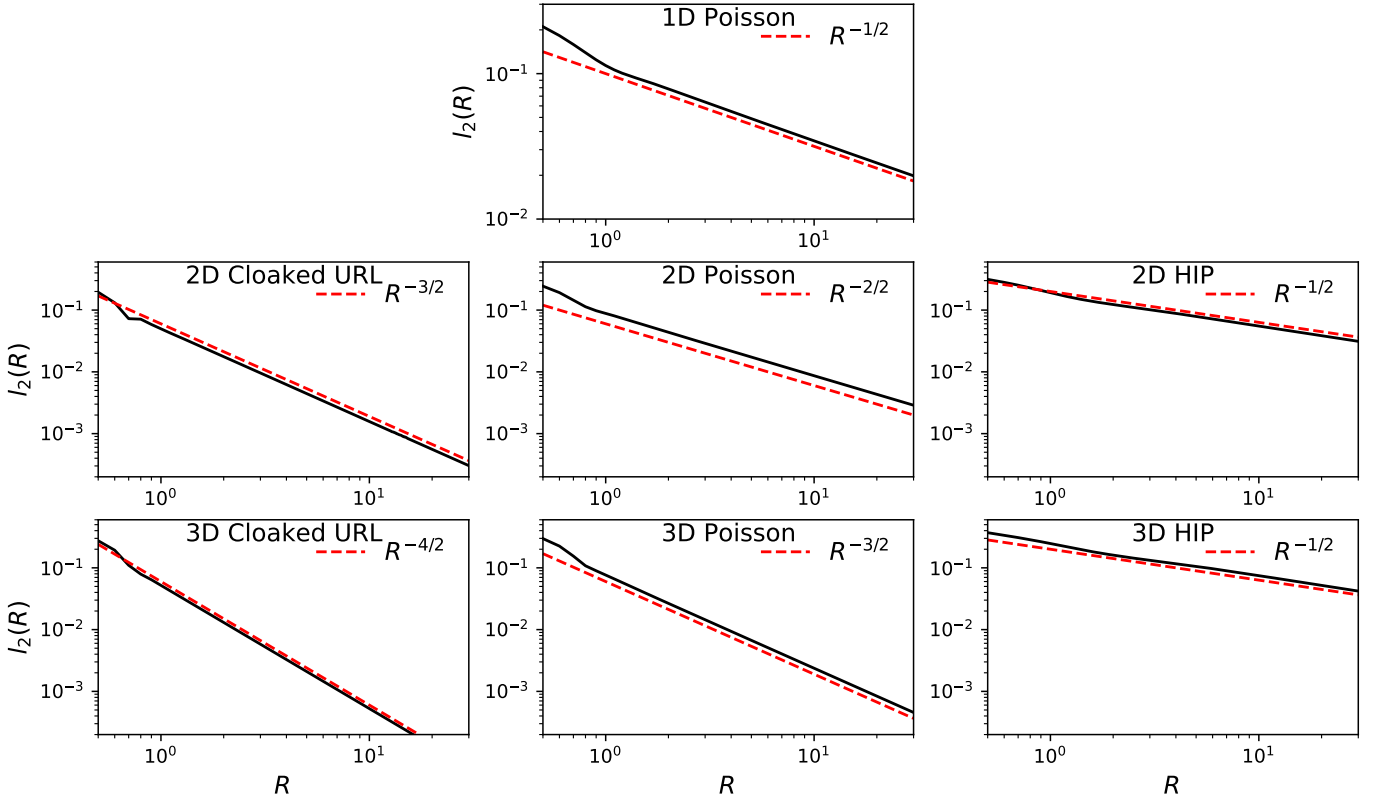

FIG. S23. Log-log plots of the  $l_2(R)$  Gaussian distance metric of the gamma-distribution approximations of  $P[N(R)]$  (black solid lines) for a representative disordered hyperuniform model (URL), nonhyperuniform model (Poisson), and anti-hyperuniform model (HIP) across the first three dimensions, respectively. The scalings of  $l_2(R)$  are in excellent agreement with those of  $|\gamma_1(R)|$  (red dashed lines) from Eq. (87) in the main article.

---

\* Email: [torquato@princeton.edu](mailto:torquato@princeton.edu)

† Email: [jaeukk@princeton.edu](mailto:jaeukk@princeton.edu)

‡ Email: [mklatt@princeton.edu](mailto:mklatt@princeton.edu)

[1] J. Kim and S. Torquato, J. Stat. Mech.: Th. and Exper. **2017**, 013402 (2017).
